# Supplementary material for: Multi-modal Representation Learning Enables Accurate Protein Function Prediction in Low-Data Setting
Source: arXiv:2412.08649 source file (2024-11-22)
Supplement: Supplementary file 1 [file HOPER_Supplementary_Material.pdf]

**Supplementary Material for:**  
**Multi-modal Representation Learning Enables Accurate Protein Function**  
**Prediction in Low-Data Setting**  
Ünsal et al., 2024

**Information About the Literature Validated Proteins Predicted to Take Part in the Immune Escape Process**

**1.1- Tumor Necrosis Factor Ligand Superfamily Member 11 (O14788)**

Tumor Necrosis Factor Ligand Superfamily Member 11 (TNFSF11=RANKL) is a cytokine belonging to the TNF alpha cytokine family that binds to the TNFRSF11A/RANK receptor. It is secreted directly by tumor tissue to create an immunosuppressive microenvironment in tumor tissues. It mediates the differentiation of T cells into suppressive Treg cells. Inhibition of this cytokine can correct the immunosuppressive microenvironment in tumor tissues and can be used in cancer treatment. Recent studies have shown that the high expression of this molecule in tumor tissues plays a role in immune evasion and can be a strategic target for tumor immunotherapy (van Dam et al. 2019).

**1.2- Proepiregulin (O14944)**

Proepiregulin is a member of the EGF-like growth factor family and is involved in cell growth and migration. Its increased expression in various cancers, such as bladder, liver, breast, lung, and colon cancers, has been shown to contribute to tumor progression. Increased epiregulin expression in lung tumors has been associated with lymph node metastasis and decreased survival. Suppression of epiregulin has been shown to decrease cell proliferation and invasion and increase apoptosis in lung tumor cells. In gastric tumors, it induces the COX-2 enzyme and increases PGE-2 production, which is one of the proteins implicated in tumor immune evasion. However, epiregulin has also been found to have indirect pro-inflammatory effects through both cytokine release and neovascularization. Thus, it is important to consider that increased epiregulin expression is associated with poor tumor prognosis and its relationship with immune evasion through COX-2 and PGE-2, but it can also exhibit pro-inflammatory effects (Riese and Cullum 2014).

**1.3- Death Receptor-6 (DR6) - a member of the Tumor Necrosis Factor Receptor Superfamily (O75509)**

Death Receptor-6 (DR6), a member of the Tumor Necrosis Factor Receptor Superfamily (TNFRSF21), can promote apoptosis via BAX-mediated release of cytochrome c from mitochondria to the cytoplasm. Increased expression of DR6 in tumor tissues has been suggested to negatively affect the maturation of dendritic cells (DCs) responsible for presenting tumor antigens to T cells, and also to reduce immature dendritic cell counts by over 50%, indicating its potential role in tumor immune evasion. Therefore, DR6

could be considered as a target in tumor immunotherapy, based on its impact on the cells that present tumor antigens (DeRosa et al. 2008).

#### **1.4- Decoy Receptor 3 (DcR3) - a member of the Tumor Necrosis Factor Receptor Superfamily (O95407)**

Decoy Receptor 3 (DcR3), also known as Tumor Necrosis Factor Receptor Superfamily member 6B (TNFRSF6B), inhibits the binding of cytotoxic ligands, TNFSF14/LIGHT, TNFSF15, and TNFSF6/FASL, to their target receptors by neutralizing them. This protein protects target cells from apoptosis and reduces T cell activity. It was identified as a protein involved in tumor immune evasion in our list of proteins and molecules involved in the phenomenon (Hsieh and Lin 2017).

#### **1.5- C-X-C motif chemokine 14 (O95715)**

C-X-C motif chemokine 14 (CXCL14) is a potent chemotactic factor for neutrophils, and also exhibits weak chemotactic properties for dendritic cells. However, it is not chemotactic for T lymphocytes, B lymphocytes, monocytes, natural killer cells, or granulocytes. A study conducted on head and neck tumors revealed decreased CXCL14 expression. In the same study, it was found that tumors in mice transfected with CXCL14 through a vector had lower volume and rate of formation than those in other mice. In another study on mice, it was observed that mice overexpressing CXCL14 were more resistant to the development of colorectal cancer, and had lower rates of metastasis to the lung and lymph nodes. These findings suggest that the increased expression of CXCL14 in tumor tissues contributes to the immune response against tumors (Yang et al. 2019).

#### **1.6- Carcinoembryonic antigen-related cell adhesion molecule 1 (P13688)**

Carcinoembryonic antigen-related cell adhesion molecule 1 (CEACAM1) suppresses T cell receptor/CD3-mediated stimulation on T lymphocytes and inhibits the cytotoxic response of T cells. It also reduces T cell proliferation and cytokine production via inhibition of the JNK cascade. CEACAM1 inhibits the activation of natural killer cells and the KLRK1-mediated cytotoxicity of target tumor cells. Additionally, it suppresses the activation of neutrophils and IL1B production.

Given its current effects, the high expression of this molecule in tumor tissue is understood to play a role in immune escape and may be a target in tumor immunotherapy (Chen et al. 2008).

#### **1.7- Matrix metalloproteinase-9 (P14780)**

Matrix metalloproteinase-9 (MMP9) cleaves collagen in the extracellular matrix, particularly types IV and V. In tumor tissue, it is produced abundantly by myeloid-derived suppressor cells (MDSCs) and plays a role in tumor angiogenesis. It also facilitates tumor invasion by increasing the number of Treg cells. In another study, MMP9 was found to increase the number of MDSCs in tumor tissue with suppressor-like

properties via osteopontin. This contributes to tumor immune escape. Based on the literature review, MMP9 can be a drug target in tumor immunotherapy due to its effects on promoting tumor angiogenesis, making the extracellular matrix conducive to tumor invasion, and contributing to tumor immune escape by increasing the number of MDSCs via osteopontin (Juric et al. 2018).

### **1.8- Insulin-like Growth Factor-Binding Protein 3 (P17936)**

Insulin-like growth factor-binding protein 3 (IGFBP3) has antiproliferative and apoptotic effects independent of IGF. It has been shown to be suppressed in many tumor tissues. IGFBP3 stimulates apoptosis in tumor cells through caspase 8, resulting in tumor suppression. These findings indicate that an increase in IGFBP3 expression has a protective effect against tumors (Ingermann et al. 2010).

### **1.9- Alpha-1-acid Glycoprotein 2 (P19652)**

Alpha-1-acid glycoprotein 2 (AGP2), also known as orosomucoid 2 (ORM2), is a protein involved in the transport of hydrophobic molecules in the blood. AGP increases the release of the cytokines IL1 beta and TNF alpha from peripheral blood mononuclear cells, which are important components of the immune response (Drenth et al. 1996). In a study of liver tumors, it was shown that ORM2 expression is lower in tumor tissue than in normal liver tissue, and this decrease is associated with poor prognosis (Zhu et al. 2020). The same study found that the decrease in ORM2 expression is associated with an increase in immune system elements with suppressive properties, such as CTLA-4, PD-L1, and TGF beta. Furthermore, it was shown that tumors with relatively higher ORM2 expression have a more effective immune response. Therefore, an increase in AGP2 expression in tumor tissue may contribute to the immune response.

### **1.10- Interleukin-11 (P20809)**

Interleukin-11 (P20809) is a member of the IL6 cytokine family that is produced by fibroblasts and endothelial cells. It reduces the release of proinflammatory cytokines, such as IL1, IL2, TNF alpha, and IFN gamma, and decreases NO production. It is used in the treatment of chemotherapy-induced thrombocytopenia in cancer patients. However, increased expression of this anti-inflammatory cytokine in tumor tissue may contribute to tumor immune escape, and this property could be targeted as a reducing strategy for this cytokine in tumor tissue in immunotherapy (Sumida et al. 2015).

### **1. 11- Tumor necrosis factor receptor superfamily member 17 (Q02223)**

Tumor necrosis factor receptor superfamily member 17 (TNFRSF17= B-cell maturation protein (BCMA)) regulates the growth, development, activation, and transformation of B lymphocytes into plasma cells. The use of monoclonal antibodies that block APRIL, a specific agonist of this receptor, has been shown to reverse the immunosuppressive tumor microenvironment and mediate antibody-dependent cell death

(ADDC) in multiple myeloma cases resistant to conventional therapy. (BCMA-targeted immunotherapy for multiple myeloma). Based on this information, it is evident that this receptor is a potential target for tumor immunotherapy (Yu, Jiang, and Liu 2020).

#### **1.12- Bcl-2-interacting killer (Q13323)**

Bcl-2-interacting killer (BIK) accelerates programmed cell death. This protein is suppressed by apoptosis inhibitors Bcl-X(L), BHRF1, and Bcl-2. It has been shown to induce apoptosis in hyperplastic cells and tumor cells (Mebratu et al. 2017). Inhibition of BIK has been found to cause epithelial cell hyperplasia and mucous cell metaplasia in smokers. This hyperplasia is the main groundwork for tumor development. Therefore, an increase in Bcl-2-interacting killer (BIK) expression is believed to prevent tumor development (Lin and Chen 2017; Mebratu et al. 2011).

#### **1.13- V-set domain-containing T-cell activation inhibitor 1 (Q7Z7D3)**

V-set domain-containing T-cell activation inhibitor 1 (VTCN1, B7-H4) is an important co-inhibitory molecule of the B7 family. In tumor tissues, VTCN1 reduces cytokine release from T cells, suppresses T cell-mediated immune responses, and supports tumor immune escape. Additionally, it plays a role in processes such as invasion, metastasis, and anti-apoptosis, leading to tumor development. In the tumor microenvironment, blocking the PD-1-PD-L1 pathway rejuvenates CD8<sup>+</sup> T cells, which have become "exhausted." However, this effect is limited in tumors such as HCC. In this case, it has been found that combining blockade of the VTCN1 (B7-H4) pathway with the PD-1-PD-L1 pathway enhances the anti-tumor immune response. Based on these findings, high expression of VTCN1 in tumor tissues is believed to play a role in immune escape and could be a promising target in tumor immunotherapy (Wang and Wang 2020; J. Li et al. 2018).

#### **1.14- Collagen triple helix repeat-containing protein 1 (Q96CG8):**

Studies have shown that increased expression of Collagen triple helix repeat-containing protein 1 (CTHRC1) contributes to tumor proliferation, invasion, and metastasis in many types of tumors. CTHRC1 exerts its effects through various pathways, such as increasing the number of suppressive M2 macrophages and activating the TGF- $\alpha$  signaling pathway by increasing smad2/smads phosphorylation, thus creating an immunosuppressive environment that may contribute to tumor immune escape. Given this information, CTHRC1's high expression in tumor tissue is understood to be involved in immune escape and may be a target in tumor immunotherapy (Mei et al. 2020; Hu et al. 2020).

#### **1.15- Hepatitis A virus cellular receptor 1 (Q96D42)**

Hepatitis A virus cellular receptor 1 (HAVcr-1), also known as CD365 or T cell immunoglobulin domain and mucin domain-1 (TIM-1), is an important member of the co-stimulator family located on the surface of

T cells. It facilitates the activation and proliferation of T cells, as well as the release of cytokines from these cells that play a role in anti-tumor response. HAVcr-1 also enhances the effectiveness of cytotoxic T lymphocytes and NK cells in the tumor microenvironment. (Immune Regulation and Antitumor Effect of TIM-1). In light of this information, increased expression of Hepatitis A virus cellular receptor 1 is understood to enhance the effectiveness of the immune system against tumors (Du et al. 2016).

#### **1.16- Atypical chemokine receptor 4 (Q9NPB9)**

It has been shown that in the absence of ACKR4 in the tumor tissue, more cytotoxic T lymphocytes collect in the tumor and kill more tumor cells, suppressing tumor growth (Whyte et al. 2020). There are also studies that show the opposite of this information. In a study by Iranian researchers, it was suggested that ACKR4 can suppress the proliferation of tumor cells (Parsi et al. 2016). In another study, it was found that ACKR4 acts as a scavenger receptor for CCL21 and ACKR4 (Ju, Sun, and Wang 2019). In this study, it has been revealed that the decrease in its expression causes an increase in the amount of CCL21 in the medium. CCL21 increase in tumor tissue mediates tumor invasion, metastasis, and tumor immune escape. Therefore, it has been revealed that the decrease in ACKR4 expression mediates the immune escape of the tumor. The reviewed literature data predominantly indicates that a decrease in ACKR4 expression will mediate tumor immune escape.

#### **1.17- Forkhead Box Protein P3 (FOXP3; Q9BZS1)**

Forkhead Box Protein P3 (FOXP3; Q9BZS1) plays a critical role as a transcriptional regulator in the development and suppressive functions of immunosuppressive Treg cells. FOXP3 was initially identified as a protein involved in tumor immune evasion and is listed as a key player in our protein and molecule list (Z. Li et al. 2015).

#### **1.18- Interleukin-23 Subunit Alpha (IL-23; Q9NPF7)**

Interleukin-23 Subunit Alpha (IL-23; Q9NPF7) shares biological activities similar to IL-12. IL-23 can enhance the proliferation of memory T cells and stimulate the production of IFN-gamma, IL-12, and TNF-alpha in activated T cells. It can also activate macrophages to produce TNF-alpha and nitric oxide and directly stimulate dendritic cells. Studies have shown that IL-23 has potent anti-tumor and anti-metastatic activity in murine cancer models. Therefore, an increase in IL-23 levels can contribute to an anti-tumor immune response (Hao and Shan 2006).

#### **1.19 - Tumor Necrosis Factor Receptor Superfamily Member 18 (Q9Y5U5)**

Tumor Necrosis Factor Receptor Superfamily Member 18 (TNFRSF18=CD357), also known as Glucocorticoid-induced TNFR-related (GITR) protein, is a receptor for TNFSF18. It regulates cell death mediated by T cell receptor (TCR) and plays a crucial role in interactions between T lymphocytes and

endothelial cells. While it is found on the surface of CD4<sup>+</sup> and CD8<sup>+</sup> T lymphocytes, it is most abundant on the surface of Treg cells. Activation of this receptor with agonists reduces the suppressive properties of Treg cells, increases CD8<sup>+</sup> T lymphocyte stimulation via CD28 and promotes their differentiation into memory cells via IL15, thereby contributing to the development of long-lasting effective responses (Durham et al. 2017; Côté et al. 2011). Clinical studies have shown that anti-tumor immune responses can be effectively activated by using agonists of this receptor (Leyland et al. 2017).

#### **1.20- Transforming Growth Factor Beta Receptor Type 3 (TGFB $\beta$ 3) (Q03167)**

TGFB $\beta$ 3, also known as betaglycan, is a type III transforming growth factor-beta receptor. Studies have shown that decreased expression of TGFB $\beta$ 3 is associated with tumor progression in prostate cancers, and correcting TGFB $\beta$ 3 levels can reduce the invasive features of tumor cells. TGFB $\beta$ 3 inhibits tumor progression by interacting with intracytoplasmic GIPC in breast cancer, suppressing TGF-beta signaling. Decreased expression of TGFB $\beta$ 3 also strengthens the TGF beta pathway and increases the accumulation of immunosuppressive Treg cells in the tumor microenvironment, contributing to immune escape. Thus, the available literature indicates that decreased TGFB $\beta$ 3 expression mediates immune escape in tumors (Turley et al. 2007; Dong et al. 1 2007; Lee et al. 2009).

**Supplementary Table S1a.** Average performance results (weighted F1-score) in terms of GO groups such as “low”, “middle”, “high”, and “specific”, “normal”, “shallow”, in ontology-based protein function prediction benchmark for GO: **(a)** molecular function, **(b)** biological process, **(c)** cellular component. “\*” sign denotes the method performs better than BLAST (considering all categories) and the difference is statistically significant (FDR<0.05).

**(a)**

| Model names           | GO-MF category |             |             |             |             |             | Methods Mean |
|-----------------------|----------------|-------------|-------------|-------------|-------------|-------------|--------------|
|                       | Low            | Middle      | High        | Specific    | Normal      | Shallow     |              |
| InterPro2GO           | 0.39           | 0.47        | 0.18        | 0.11        | 0.46        | 0.45        | 0.35         |
| UniRule2GO            | 0.01           | 0.01        | 0.01        | 0.00        | 0.02        | 0.01        | 0.01         |
| Ensembl-Orthology     | 0.15           | 0.25        | 0.20        | 0.14        | 0.21        | 0.23        | 0.20         |
| BLAST                 | 0.86           | 0.89        | 0.88        | 0.90        | 0.91        | 0.82        | 0.88         |
| HMMER                 | <b>0.89</b>    | 0.89        | 0.88        | <b>0.92</b> | 0.91        | 0.85        | 0.89         |
| K-Sep                 | 0.82           | 0.81        | 0.79        | 0.84        | 0.85        | 0.75        | 0.81         |
| APAAC                 | 0.65           | 0.49        | 0.62        | 0.51        | 0.70        | 0.51        | 0.58         |
| PFAM                  | 0.85           | 0.86        | 0.88        | 0.84        | 0.89        | 0.86        | 0.86         |
| AAC                   | 0.37           | 0.36        | 0.55        | 0.26        | 0.59        | 0.33        | 0.41         |
| ProtVec               | 0.67           | 0.55        | 0.71        | 0.57        | 0.72        | 0.59        | 0.64         |
| Gene2Vec              | 0.52           | 0.60        | 0.45        | 0.48        | 0.65        | 0.44        | 0.52         |
| Learned-Vec           | 0.66           | 0.66        | 0.71        | 0.63        | 0.75        | 0.63        | 0.68         |
| Mut2Vec               | 0.50           | 0.60        | 0.64        | 0.54        | 0.65        | 0.52        | 0.58         |
| TCGA-Embedding        | 0.36           | 0.35        | 0.30        | 0.35        | 0.48        | 0.20        | 0.34         |
| SeqVec                | 0.86           | <b>0.91</b> | 0.90        | 0.91        | 0.91        | 0.85        | 0.89         |
| MSA-Transformer       | 0.55           | 0.71        | 0.78        | 0.72        | 0.71        | 0.59        | 0.68         |
| CPCProt               | 0.64           | 0.61        | 0.74        | 0.61        | 0.75        | 0.59        | 0.66         |
| ProtBERT-BFD          | 0.82           | 0.86        | 0.88        | 0.85        | 0.85        | 0.84        | 0.85         |
| TAPE-BERT-PFAM        | 0.83           | 0.86        | 0.85        | 0.86        | 0.87        | 0.82        | 0.85         |
| ESM-1b                | 0.80           | 0.85        | 0.85        | 0.85        | 0.89        | 0.76        | 0.83         |
| ProtALBERT            | 0.86           | 0.90        | 0.90        | 0.89        | 0.90        | <b>0.87</b> | 0.89         |
| ProtXLNet             | 0.79           | 0.82        | 0.84        | 0.84        | 0.84        | 0.78        | 0.82         |
| UniRep                | 0.85           | 0.80        | 0.83        | 0.86        | 0.87        | 0.75        | 0.83         |
| ProtT5-XL             | <b>0.89</b>    | <b>0.91</b> | <b>0.92</b> | <b>0.92</b> | <b>0.93</b> | 0.86        | <b>0.90</b>  |
| <b>Category Mean:</b> | 0.65           | 0.67        | 0.68        | 0.64        | 0.72        | 0.62        | 0.66         |

(b)

| Model names       | GO-BP category |             |             |             |             |             | Method Mean |
|-------------------|----------------|-------------|-------------|-------------|-------------|-------------|-------------|
|                   | Low            | Middle      | High        | Specific    | Normal      | Shallow     |             |
| InterPro2GO       | 0.18           | 0.10        | 0.06        | 0.08        | 0.15        | 0.10        | 0.11        |
| UniRule2GO        | 0.03           | 0.00        | 0.00        | 0.02        | 0.01        | 0.00        | 0.01        |
| Ensembl-Orthology | 0.23           | 0.36        | 0.13        | 0.25        | 0.27        | 0.20        | 0.24        |
| BLAST             | 0.36           | 0.68        | 0.63        | 0.63        | 0.48        | 0.56        | 0.56        |
| HMMER*            | <b>0.52</b>    | 0.69        | 0.63        | 0.67        | 0.56        | 0.60        | 0.61        |
| K-Sep             | 0.47           | 0.60        | 0.48        | 0.61        | 0.46        | 0.48        | 0.52        |
| APAAC             | 0.29           | 0.41        | 0.34        | 0.46        | 0.26        | 0.32        | 0.34        |
| PFAM              | 0.37           | 0.67        | 0.63        | 0.62        | 0.52        | 0.53        | 0.56        |
| AAC               | 0.15           | 0.27        | 0.14        | 0.25        | 0.13        | 0.18        | 0.19        |
| ProtVec           | 0.32           | 0.42        | 0.34        | 0.51        | 0.30        | 0.28        | 0.36        |
| Gene2Vec          | 0.38           | 0.52        | 0.41        | 0.47        | 0.42        | 0.42        | 0.44        |
| Learned-Vec       | 0.40           | 0.46        | 0.32        | 0.55        | 0.28        | 0.35        | 0.39        |
| Mut2Vec           | 0.29           | 0.49        | 0.50        | 0.52        | 0.36        | 0.40        | 0.43        |
| TCGA-Embedding    | 0.37           | 0.37        | 0.22        | 0.37        | 0.31        | 0.28        | 0.32        |
| SeqVec            | 0.45           | 0.73        | 0.62        | 0.68        | 0.55        | 0.57        | 0.60        |
| MSA-Transformer   | 0.38           | 0.53        | 0.50        | 0.57        | 0.41        | 0.43        | 0.47        |
| CPCProt           | 0.32           | 0.48        | 0.39        | 0.48        | 0.33        | 0.37        | 0.40        |
| ProtBERT-BFD      | <b>0.52</b>    | 0.69        | 0.62        | 0.69        | 0.58        | 0.57        | 0.61        |
| TAPE-BERT-PFAM    | 0.48           | 0.63        | 0.50        | 0.65        | 0.51        | 0.44        | 0.54        |
| ESM-1b            | 0.35           | 0.65        | 0.59        | 0.58        | 0.52        | 0.49        | 0.53        |
| ProtALBERT*       | 0.47           | 0.74        | <b>0.67</b> | 0.65        | <b>0.64</b> | 0.59        | 0.63        |
| ProtXLNet         | 0.33           | 0.60        | 0.56        | 0.58        | 0.48        | 0.44        | 0.50        |
| UniRep            | 0.42           | 0.59        | 0.43        | 0.59        | 0.44        | 0.41        | 0.48        |
| ProtT5-XL*        | <b>0.52</b>    | <b>0.78</b> | <b>0.67</b> | <b>0.72</b> | 0.60        | <b>0.65</b> | <b>0.66</b> |
| Category Mean:    | 0.36           | 0.52        | 0.43        | 0.51        | 0.40        | 0.40        | 0.44        |

(c)

| Methods           | GO category |             |             |             |             |             | Method Mean |
|-------------------|-------------|-------------|-------------|-------------|-------------|-------------|-------------|
|                   | Low         | Middle      | High        | Specific    | Normal      | Shallow     |             |
| InterPro2GO       | 0.34        | 0.14        | 0.37        | 0.17        | 0.16        | 0.45        | 0.27        |
| UniRule2GO        | 0.00        | 0.05        | 0.08        | 0.04        | 0.05        | 0.03        | 0.04        |
| Ensembl-Orthology | 0.23        | 0.26        | 0.32        | 0.20        | 0.27        | 0.30        | 0.26        |
| BLAST             | 0.46        | 0.59        | 0.71        | 0.44        | 0.64        | 0.59        | 0.57        |
| HMMER             | 0.52        | 0.61        | 0.69        | 0.47        | 0.65        | 0.63        | 0.59        |
| K-Sep             | 0.41        | 0.56        | 0.56        | 0.48        | 0.50        | 0.52        | 0.50        |
| APAAC             | 0.35        | 0.41        | 0.44        | 0.35        | 0.39        | 0.43        | 0.40        |
| PFAM              | 0.47        | 0.61        | 0.70        | 0.45        | 0.64        | 0.61        | 0.58        |
| AAC               | 0.13        | 0.21        | 0.43        | 0.11        | 0.27        | 0.27        | 0.24        |
| ProtVec           | 0.26        | 0.42        | 0.50        | 0.26        | 0.41        | 0.43        | 0.38        |
| Gene2Vec          | 0.43        | 0.56        | 0.52        | 0.46        | 0.52        | 0.50        | 0.50        |
| Learned-Vec       | 0.30        | 0.46        | 0.50        | 0.28        | 0.44        | 0.46        | 0.41        |
| Mut2Vec           | 0.37        | 0.50        | 0.54        | 0.47        | 0.44        | 0.48        | 0.47        |
| TCGA-Embedding    | 0.35        | 0.43        | 0.47        | 0.33        | 0.49        | 0.39        | 0.41        |
| SeqVec            | 0.49        | 0.66        | 0.70        | 0.49        | 0.62        | 0.67        | 0.61        |
| MSA-Transformer   | 0.36        | 0.55        | 0.64        | 0.36        | 0.57        | 0.54        | 0.50        |
| CPCProt           | 0.32        | 0.47        | 0.55        | 0.35        | 0.47        | 0.46        | 0.44        |
| ProtBERT-BFD      | 0.53        | 0.67        | 0.69        | 0.49        | 0.67        | 0.67        | 0.62        |
| TAPE-BERT-PFAM    | 0.50        | 0.63        | 0.62        | 0.51        | 0.61        | 0.60        | 0.58        |
| ESM-1b            | 0.51        | 0.64        | 0.71        | 0.54        | 0.60        | 0.67        | 0.61        |
| ProtALBERT*       | 0.54        | 0.67        | 0.73        | 0.51        | 0.66        | 0.70        | 0.63        |
| ProtXLNet         | 0.50        | 0.63        | 0.66        | 0.47        | 0.61        | 0.64        | 0.59        |
| UniRep            | 0.45        | 0.56        | 0.61        | 0.41        | 0.58        | 0.57        | 0.53        |
| ProtT5-XL*        | <b>0.58</b> | <b>0.74</b> | <b>0.74</b> | <b>0.57</b> | <b>0.69</b> | <b>0.75</b> | <b>0.68</b> |
| Category Mean:    | 0.39        | 0.50        | 0.56        | 0.38        | 0.50        | 0.51        | 0.48        |

**Supplementary Table S1b.** Average performance results of protein-protein interaction-based representation models (weighted F1 score). Results are measured in "low", "middle", "high" and "specific", "normal", "shallow" groups. (a) Molecular Function, (b) Biological Processes, and (c) Cellular Component.

(a)

|                             | GO-MF category |             |             |             |             |             |             |
|-----------------------------|----------------|-------------|-------------|-------------|-------------|-------------|-------------|
| Method names                | Low            | Middle      | High        | Specific    | Normal      | Shallow     | Method Mean |
| node2vec_d_200_p_2_q_0.25   | <b>0.59</b>    | 0.60        | 0.61        | <b>0.72</b> | 0.66        | 0.50        | <b>0.61</b> |
| node2vec_d_500_p_0.5_q_0.25 | <b>0.59</b>    | 0.59        | <b>0.63</b> | 0.65        | <b>0.68</b> | 0.50        | <b>0.61</b> |
| node2vec_d_1000_p_2_q_0.25  | 0.56           | 0.60        | 0.61        | 0.69        | 0.62        | <b>0.53</b> | 0.60        |
| node2vec_d_100_p_0.25_q_0.5 | 0.54           | 0.59        | <b>0.63</b> | 0.69        | 0.64        | 0.50        | 0.60        |
| node2vec_d_500_p_2_q_0.25   | 0.52           | <b>0.61</b> | 0.62        | 0.68        | 0.63        | 0.52        | 0.60        |
| node2vec_d_100_p_0.5_q_1    | 0.58           | 0.57        | <b>0.63</b> | 0.64        | 0.63        | 0.52        | 0.59        |
| node2vec_d_1000_p_2_q_0.5   | 0.56           | 0.59        | 0.61        | 0.66        | 0.66        | 0.49        | 0.59        |
| node2vec_d_1000_p_2_q_1     | 0.53           | 0.60        | 0.62        | 0.67        | 0.64        | 0.51        | 0.59        |
| node2vec_d_500_p_1_q_2      | 0.54           | 0.60        | 0.61        | 0.66        | 0.65        | 0.50        | 0.59        |
| node2vec_d_100_p_2_q_0.5    | 0.58           | 0.57        | 0.62        | 0.60        | 0.65        | 0.52        | 0.59        |
| HOPE_d_1000_beta_0.125      | 0.27           | 0.29        | 0.33        | 0.37        | 0.36        | 0.20        | 0.30        |
| HOPE_d_1000_beta_0.25       | 0.24           | 0.31        | 0.34        | 0.35        | 0.36        | 0.22        | 0.30        |
| HOPE_d_500_beta_0.25        | 0.23           | 0.32        | 0.30        | 0.38        | 0.33        | 0.22        | 0.30        |
| HOPE_d_200_beta_0.25        | 0.25           | 0.29        | 0.26        | 0.34        | 0.37        | 0.15        | 0.28        |
| HOPE_d_500_beta_0.0625      | 0.26           | 0.27        | 0.25        | 0.36        | 0.30        | 0.19        | 0.27        |
| HOPE_d_200_beta_0.125       | 0.26           | 0.25        | 0.27        | 0.32        | 0.33        | 0.18        | 0.27        |

|                         |             |             |             |             |             |             |             |
|-------------------------|-------------|-------------|-------------|-------------|-------------|-------------|-------------|
| HOPE_d_100_beta_0.25    | 0.20        | 0.28        | 0.27        | 0.38        | 0.33        | 0.14        | 0.27        |
| HOPE_d_200_beta_0.0625  | 0.29        | 0.25        | 0.23        | 0.33        | 0.33        | 0.16        | 0.26        |
| HOPE_d_500_beta_0.125   | 0.18        | 0.27        | 0.29        | 0.31        | 0.31        | 0.17        | 0.25        |
| HOPE_d_1000_beta_0.0625 | 0.24        | 0.22        | 0.28        | 0.25        | 0.29        | 0.19        | 0.25        |
| Category Average        | <b>0.40</b> | <b>0.43</b> | <b>0.45</b> | <b>0.50</b> | <b>0.49</b> | <b>0.34</b> | <b>0.44</b> |

(b)

|                              | GO-BP category |             |             |             |             |             |             |
|------------------------------|----------------|-------------|-------------|-------------|-------------|-------------|-------------|
| Method names                 | Low            | Middle      | High        | Specific    | Normal      | Shallow     | Method Mean |
| node2vec_d_1000_p_2_q_1      | 0.42           | 0.62        | 0.50        | 0.54        | 0.52        | 0.47        | <b>0.51</b> |
| node2vec_d_200_p_1_q_2       | 0.39           | <b>0.64</b> | 0.51        | 0.54        | 0.51        | <b>0.49</b> | 0.51        |
| node2vec_d_500_p_2_q_2       | 0.39           | 0.62        | <b>0.52</b> | <b>0.57</b> | 0.50        | 0.46        | 0.51        |
| node2vec_d_500_p_1_q_2       | 0.39           | 0.62        | 0.51        | 0.54        | 0.52        | 0.46        | 0.51        |
| node2vec_d_100_p_0.25_q_0.25 | 0.40           | 0.62        | 0.50        | <b>0.57</b> | 0.49        | 0.47        | 0.51        |
| node2vec_d_500_p_0.5_q_2     | <b>0.43</b>    | 0.61        | 0.48        | 0.53        | <b>0.54</b> | 0.46        | 0.51        |
| node2vec_d_500_p_1_q_1       | 0.41           | 0.62        | 0.49        | 0.55        | 0.52        | 0.46        | 0.51        |
| node2vec_d_500_p_2_q_1       | 0.40           | 0.61        | 0.50        | 0.52        | <b>0.54</b> | 0.44        | 0.50        |
| node2vec_d_50_p_1_q_2        | <b>0.43</b>    | 0.61        | 0.46        | 0.54        | 0.51        | 0.44        | 0.50        |
| node2vec_d_500_p_0.5_q_0.25  | 0.38           | 0.61        | 0.50        | 0.53        | 0.52        | 0.45        | 0.50        |
| HOPE_d_1000_beta_0.25        | 0.27           | 0.29        | 0.23        | 0.36        | 0.21        | 0.22        | 0.26        |
| HOPE_d_500_beta_0.25         | 0.29           | 0.28        | 0.17        | 0.33        | 0.23        | 0.19        | 0.25        |
| HOPE_d_1000_beta_0.5         | 0.21           | 0.30        | 0.21        | 0.32        | 0.14        | 0.25        | 0.24        |
| HOPE_d_200_beta_0.25         | 0.30           | 0.26        | 0.14        | 0.32        | 0.18        | 0.20        | 0.23        |

|                         |             |             |             |             |             |             |             |
|-------------------------|-------------|-------------|-------------|-------------|-------------|-------------|-------------|
| HOPE_d_1000_beta_0.125  | 0.20        | 0.28        | 0.22        | 0.31        | 0.19        | 0.19        | 0.23        |
| HOPE_d_100_beta_0.25    | 0.31        | 0.25        | 0.11        | 0.30        | 0.19        | 0.19        | 0.23        |
| HOPE_d_500_beta_0.125   | 0.21        | 0.28        | 0.16        | 0.27        | 0.19        | 0.18        | 0.21        |
| HOPE_d_500_beta_0.0625  | 0.24        | 0.26        | 0.13        | 0.26        | 0.16        | 0.22        | 0.21        |
| HOPE_d_500_beta_0.5     | 0.20        | 0.28        | 0.15        | 0.30        | 0.10        | 0.23        | 0.21        |
| HOPE_d_1000_beta_0.0625 | 0.26        | 0.24        | 0.13        | 0.24        | 0.17        | 0.21        | 0.21        |
| <b>Category Average</b> | <b>0.33</b> | <b>0.44</b> | <b>0.33</b> | <b>0.42</b> | <b>0.35</b> | <b>0.33</b> | <b>0.37</b> |

(c)

|                              | GO-CC category |             |             |             |             |             |             |
|------------------------------|----------------|-------------|-------------|-------------|-------------|-------------|-------------|
| Method names                 | Low            | Middle      | High        | Specific    | Normal      | Shallow     | Method Mean |
| node2vec_d_1000_p_1_q_2      | 0.55           | <b>0.66</b> | 0.64        | 0.59        | <b>0.59</b> | 0.64        | <b>0.61</b> |
| node2vec_d_1000_p_0.25_q_0.5 | 0.54           | 0.63        | 0.64        | <b>0.60</b> | 0.58        | 0.62        | 0.60        |
| node2vec_d_200_p_2_q_1       | <b>0.56</b>    | 0.63        | 0.61        | 0.55        | 0.57        | <b>0.66</b> | 0.60        |
| node2vec_d_1000_p_2_q_0.5    | 0.52           | 0.63        | <b>0.65</b> | 0.56        | 0.56        | 0.64        | 0.59        |
| node2vec_d_1000_p_2_q_1      | 0.51           | 0.64        | 0.64        | 0.57        | 0.55        | 0.64        | 0.59        |
| node2vec_d_1000_p_0.25_q_1   | 0.50           | 0.64        | 0.63        | 0.58        | 0.55        | 0.62        | 0.59        |
| node2vec_d_1000_p_0.5_q_1    | 0.51           | 0.62        | 0.64        | 0.55        | 0.55        | 0.65        | 0.59        |
| node2vec_d_1000_p_0.5_q_0.5  | 0.51           | 0.63        | 0.64        | 0.57        | 0.56        | 0.62        | 0.59        |
| node2vec_d_500_p_2_q_2       | 0.50           | 0.65        | 0.63        | 0.54        | 0.57        | 0.64        | 0.59        |
| node2vec_d_500_p_2_q_1       | 0.50           | 0.64        | 0.64        | 0.52        | 0.57        | 0.65        | 0.59        |
| HOPE_d_500_beta_0.0625       | 0.33           | 0.34        | 0.43        | 0.27        | 0.35        | 0.42        | 0.35        |

|                         |             |             |             |             |             |             |             |
|-------------------------|-------------|-------------|-------------|-------------|-------------|-------------|-------------|
| HOPE_d_1000_beta_0.0625 | 0.35        | 0.30        | 0.43        | 0.33        | 0.34        | 0.38        | 0.35        |
| HOPE_d_500_beta_0.125   | 0.27        | 0.34        | 0.42        | 0.25        | 0.36        | 0.37        | 0.33        |
| HOPE_d_500_beta_0.25    | 0.25        | 0.35        | 0.42        | 0.23        | 0.39        | 0.34        | 0.33        |
| HOPE_d_100_beta_0.125   | 0.27        | 0.30        | 0.42        | 0.24        | 0.35        | 0.34        | 0.32        |
| HOPE_d_1000_beta_0.25   | 0.21        | 0.36        | 0.43        | 0.21        | 0.39        | 0.33        | 0.32        |
| HOPE_d_1000_beta_0.125  | 0.21        | 0.34        | 0.43        | 0.24        | 0.36        | 0.32        | 0.32        |
| HOPE_d_200_beta_0.125   | 0.24        | 0.32        | 0.42        | 0.22        | 0.36        | 0.34        | 0.32        |
| HOPE_d_200_beta_0.0625  | 0.28        | 0.27        | 0.42        | 0.24        | 0.34        | 0.34        | 0.32        |
| HOPE_d_200_beta_0.25    | 0.22        | 0.34        | 0.42        | 0.20        | 0.39        | 0.32        | 0.32        |
| Category Average        | <b>0.39</b> | <b>0.48</b> | <b>0.53</b> | <b>0.40</b> | <b>0.46</b> | <b>0.49</b> | <b>0.46</b> |

**Supplementary Table S1c.** Average performance results of protein text-based representation models (weighted F1 score). Results are measured in "low", "middle", "high" and "specific", "normal", "shallow" groups. (a) Molecular Function, (b) Biological Processes, and (c) Cellular Component.

(a)

|                                | GO-MF category |             |             |             |             |             |             |
|--------------------------------|----------------|-------------|-------------|-------------|-------------|-------------|-------------|
| Method names                   | Low            | Middle      | High        | Specific    | Normal      | Shallow     | Method Mean |
| TF-IDF_PCA-1024-PUBMED-UNIPROT | <b>0.91</b>    | 0.89        | <b>0.89</b> | <b>0.91</b> | <b>0.91</b> | <b>0.88</b> | <b>0.90</b> |
| TF-IDF_PCA-512-PUBMED-UNIPROT  | 0.84           | <b>0.90</b> | 0.87        | 0.90        | 0.90        | 0.83        | 0.87        |
| TF-IDF_PCA-256-PUBMED-UNIPROT  | 0.85           | 0.87        | 0.86        | 0.88        | <b>0.91</b> | 0.79        | 0.86        |
| BIOSENTVEC-UNIPROT             | 0.82           | 0.88        | 0.85        | 0.87        | <b>0.91</b> | 0.78        | 0.85        |
| BIOSENTVEC-PUBMED-UNIPROT      | 0.80           | 0.88        | 0.87        | 0.86        | 0.89        | 0.80        | 0.85        |

|                             |             |             |             |             |             |             |             |
|-----------------------------|-------------|-------------|-------------|-------------|-------------|-------------|-------------|
| TF-IDF_PCA-1024-UNIPROT     | 0.78        | 0.90        | 0.87        | 0.78        | 0.92        | 0.82        | 0.85        |
| TF-IDF_PCA-256-UNIPROT      | 0.81        | 0.87        | 0.86        | 0.83        | 0.90        | 0.80        | 0.85        |
| BIOBERT-UNIPROT-AVG         | 0.74        | 0.80        | 0.82        | 0.80        | 0.84        | 0.70        | 0.78        |
| BIOWORDVEC-UNIPROT          | 0.74        | 0.80        | 0.82        | 0.79        | 0.87        | 0.69        | 0.78        |
| BIOBERT-PUBMED-UNIPROT-AVG  | 0.61        | 0.76        | 0.80        | 0.78        | 0.76        | 0.63        | 0.72        |
| BIOWORDVEC-PUBMED-UNIPROT   | 0.47        | 0.65        | 0.69        | 0.53        | 0.66        | 0.57        | 0.59        |
| BIOBERT-UNIPROT-POOL        | 0.37        | 0.56        | 0.71        | 0.47        | 0.61        | 0.48        | 0.53        |
| BIOBERT-PUBMED-UNIPROT-POOL | 0.34        | 0.45        | 0.67        | 0.30        | 0.57        | 0.47        | 0.47        |
| Category Average            | <b>0.70</b> | <b>0.79</b> | <b>0.82</b> | <b>0.75</b> | <b>0.82</b> | <b>0.71</b> | <b>0.76</b> |

(b)

|                                | GO-BP category |             |             |             |             |             |             |
|--------------------------------|----------------|-------------|-------------|-------------|-------------|-------------|-------------|
| Method names                   | Low            | Middle      | High        | Specific    | Normal      | Shallow     | Method Mean |
| TF-IDF_PCA-512-PUBMED-UNIPROT  | <b>0.69</b>    | 0.86        | 0.75        | 0.80        | <b>0.74</b> | <b>0.77</b> | <b>0.77</b> |
| TF-IDF_PCA-1024-PUBMED-UNIPROT | 0.67           | <b>0.87</b> | <b>0.76</b> | 0.80        | 0.72        | <b>0.77</b> | 0.76        |
| TF-IDF_PCA-256-PUBMED-UNIPROT  | 0.68           | 0.85        | 0.73        | 0.79        | 0.71        | 0.76        | 0.75        |
| BIOSENTVEC-PUBMED-UNIPROT      | 0.68           | 0.84        | 0.74        | 0.77        | 0.73        | 0.76        | 0.75        |
| TF-IDF_PCA-256-UNIPROT         | 0.59           | 0.85        | 0.73        | 0.82        | 0.63        | 0.71        | 0.72        |
| BIOSENTVEC-UNIPROT             | 0.58           | 0.84        | 0.73        | 0.79        | 0.69        | 0.68        | 0.72        |
| TF-IDF_PCA-1024-UNIPROT        | 0.53           | 0.86        | <b>0.76</b> | <b>0.83</b> | 0.65        | 0.66        | 0.72        |
| BIOWORDVEC-UNIPROT             | 0.46           | 0.79        | 0.70        | 0.76        | 0.56        | 0.64        | 0.65        |

|                             |             |             |             |             |             |             |             |
|-----------------------------|-------------|-------------|-------------|-------------|-------------|-------------|-------------|
| BIOBERT-UNIPROT-AVG         | 0.44        | 0.79        | 0.70        | 0.75        | 0.61        | 0.56        | 0.64        |
| BIOBERT-PUBMED-UNIPROT-AVG  | 0.29        | 0.65        | 0.66        | 0.57        | 0.46        | 0.57        | 0.53        |
| BIOWORDVEC-PUBMED-UNIPROT   | 0.33        | 0.60        | 0.53        | 0.56        | 0.43        | 0.47        | 0.49        |
| BIOBERT-UNIPROT-POOL        | 0.31        | 0.53        | 0.53        | 0.51        | 0.46        | 0.41        | 0.46        |
| BIOBERT-PUBMED-UNIPROT-POOL | 0.20        | 0.44        | 0.50        | 0.48        | 0.30        | 0.36        | 0.38        |
| Category Average            | <b>0.50</b> | <b>0.75</b> | <b>0.68</b> | <b>0.71</b> | <b>0.59</b> | <b>0.62</b> | <b>0.64</b> |

(c)

|                                | GO-CC category |             |             |             |             |             |             |
|--------------------------------|----------------|-------------|-------------|-------------|-------------|-------------|-------------|
| Method names                   | Low            | Middle      | High        | Specific    | Normal      | Shallow     | Method Mean |
| TF-IDF_PCA-512-PUBMED-UNIPROT  | 0.81           | <b>0.82</b> | 0.75        | <b>0.75</b> | 0.79        | <b>0.85</b> | <b>0.79</b> |
| TF-IDF_PCA-1024-PUBMED-UNIPROT | <b>0.82</b>    | 0.81        | <b>0.76</b> | 0.72        | <b>0.81</b> | <b>0.85</b> | <b>0.79</b> |
| TF-IDF_PCA-256-PUBMED-UNIPROT  | <b>0.82</b>    | 0.79        | 0.73        | 0.73        | 0.79        | 0.82        | 0.78        |
| BIOSENTVEC-PUBMED-UNIPROT      | 0.73           | 0.80        | 0.74        | 0.70        | 0.76        | 0.79        | 0.75        |
| BIOSENTVEC-UNIPROT             | 0.75           | 0.79        | 0.72        | 0.69        | 0.76        | 0.80        | 0.75        |
| TF-IDF_PCA-1024-UNIPROT        | 0.73           | 0.80        | 0.74        | 0.67        | 0.76        | 0.81        | 0.75        |
| TF-IDF_PCA-256-UNIPROT         | 0.73           | 0.80        | 0.72        | 0.68        | 0.77        | 0.77        | 0.75        |
| BIOWORDVEC-UNIPROT             | 0.64           | 0.73        | 0.63        | 0.61        | 0.64        | 0.75        | 0.66        |
| BIOBERT-UNIPROT-AVG            | 0.54           | 0.74        | 0.67        | 0.58        | 0.65        | 0.69        | 0.65        |
| BIOBERT-PUBMED-UNIPROT-AVG     | 0.44           | 0.68        | 0.68        | 0.47        | 0.60        | 0.66        | 0.59        |

|                                    |             |             |             |             |             |             |             |
|------------------------------------|-------------|-------------|-------------|-------------|-------------|-------------|-------------|
| <b>BIOWORDVEC-PUBMED-UNIPROT</b>   | 0.39        | 0.56        | 0.54        | 0.31        | 0.49        | 0.61        | 0.48        |
| <b>BIOBERT-UNIPROT-POOL</b>        | 0.27        | 0.54        | 0.60        | 0.33        | 0.50        | 0.49        | 0.45        |
| <b>BIOBERT-PUBMED-UNIPROT-POOL</b> | 0.27        | 0.51        | 0.60        | 0.31        | 0.49        | 0.49        | 0.44        |
| <b>Category Average</b>            | <b>0.61</b> | <b>0.72</b> | <b>0.68</b> | <b>0.58</b> | <b>0.68</b> | <b>0.72</b> | <b>0.67</b> |

**Supplementary Table S2.** Average performance results of multimodal representation models (weighted F1 score). Results are measured in "low", "middle", "high" and "specific", "normal", "shallow" groups. (a) Molecular Function, (b) Biological Processes, and (c) Cellular Component.

(a)

|                                      | GO-MF category |             |             |             |             |             |             |
|--------------------------------------|----------------|-------------|-------------|-------------|-------------|-------------|-------------|
| Method names                         | Low            | Middle      | High        | Specific    | Normal      | Shallow     | Method Mean |
| <b>SimpleAE_512</b>                  | <b>0.93</b>    | <b>0.93</b> | 0.90        | <b>0.97</b> | <b>0.95</b> | 0.88        | <b>0.93</b> |
| <b>Simple AE_1024</b>                | <b>0.93</b>    | 0.92        | 0.88        | 0.94        | 0.93        | <b>0.89</b> | 0.92        |
| <b>MultiModalAE_768</b>              | 0.92           | 0.92        | 0.89        | 0.93        | 0.94        | 0.88        | 0.91        |
| <b>SimpleAE_256</b>                  | 0.88           | <b>0.93</b> | 0.90        | 0.95        | 0.93        | 0.87        | 0.91        |
| <b>SimpleAE_768</b>                  | 0.91           | 0.92        | 0.89        | 0.94        | 0.93        | 0.87        | 0.91        |
| <b>MultiModalAE_1024</b>             | 0.91           | 0.92        | 0.89        | 0.93        | 0.93        | 0.88        | 0.91        |
| <b>TransferAE_768</b>                | 0.92           | 0.92        | 0.88        | 0.93        | 0.93        | 0.87        | 0.91        |
| <b>MultiModalAE_256</b>              | 0.90           | 0.91        | 0.89        | 0.94        | 0.94        | 0.86        | 0.91        |
| <b>T5_TF-IDF_PCA</b>                 | 0.86           | 0.92        | 0.92        | 0.92        | 0.92        | 0.88        | 0.91        |
| <b>TF-IDF_PCA</b>                    | 0.91           | 0.91        | 0.88        | 0.92        | 0.92        | 0.88        | 0.90        |
| <b>TransferAE_512</b>                | 0.91           | 0.90        | 0.87        | 0.93        | 0.93        | 0.86        | 0.90        |
| <b>Multi_Modal AE_Seq_Based_1024</b> | 0.88           | 0.91        | 0.88        | 0.94        | 0.92        | 0.86        | 0.90        |
| <b>TransferAE_256</b>                | 0.89           | 0.91        | 0.87        | 0.93        | 0.91        | 0.86        | 0.89        |
| <b>T5</b>                            | 0.85           | 0.91        | <b>0.91</b> | 0.90        | 0.91        | 0.87        | 0.89        |

|                     |             |             |             |             |             |             |             |
|---------------------|-------------|-------------|-------------|-------------|-------------|-------------|-------------|
| T5_NODE2VEC_TF-IDF  | 0.73        | 0.90        | 0.90        | 0.86        | 0.86        | 0.83        | 0.85        |
| T5_NODE2VEC         | 0.72        | 0.88        | 0.89        | 0.85        | 0.85        | 0.81        | 0.83        |
| NODE2VEC_TF-IDF_PCA | 0.64        | 0.76        | 0.81        | 0.71        | 0.75        | 0.73        | 0.73        |
| NODE2VEC            | 0.57        | 0.54        | 0.58        | 0.58        | 0.64        | 0.47        | 0.57        |
| Category Average    | <b>0.85</b> | <b>0.88</b> | <b>0.87</b> | <b>0.89</b> | <b>0.89</b> | <b>0.84</b> | <b>0.87</b> |

(b)

|                        | GO-BP category |             |             |             |             |             |             |
|------------------------|----------------|-------------|-------------|-------------|-------------|-------------|-------------|
| Method names           | Low            | Middle      | High        | Specific    | Normal      | Shallow     | Method Mean |
| TF-IDF                 | 0.74           | <b>0.86</b> | <b>0.76</b> | <b>0.80</b> | <b>0.80</b> | <b>0.76</b> | <b>0.79</b> |
| MultiModalAE_768       | 0.75           | 0.81        | 0.69        | 0.76        | 0.77        | 0.72        | 0.75        |
| MultiModalAE_256       | <b>0.76</b>    | 0.80        | 0.69        | 0.74        | 0.79        | 0.72        | 0.75        |
| MultiModalAE_1024      | 0.74           | 0.82        | 0.69        | 0.76        | 0.77        | 0.71        | 0.75        |
| SimpleAE_1024          | 0.73           | 0.82        | 0.69        | 0.76        | 0.76        | 0.72        | 0.75        |
| SimpleAE_768           | 0.72           | 0.82        | 0.68        | 0.75        | 0.76        | 0.71        | 0.74        |
| SimpleAE_512           | 0.70           | 0.83        | 0.68        | 0.74        | 0.75        | 0.71        | 0.73        |
| T5_TF-IDF_PCA          | 0.60           | 0.83        | 0.76        | 0.75        | 0.72        | 0.72        | 0.73        |
| SimpleAE_256           | 0.67           | 0.83        | 0.68        | 0.75        | 0.72        | 0.71        | 0.73        |
| TransferAE_256         | 0.69           | 0.77        | 0.64        | 0.72        | 0.71        | 0.66        | 0.70        |
| TransferAE_768         | 0.68           | 0.78        | 0.62        | 0.73        | 0.69        | 0.66        | 0.69        |
| TransferAE_1024        | 0.67           | 0.77        | 0.62        | 0.73        | 0.70        | 0.64        | 0.69        |
| TransferAE_512         | 0.67           | 0.78        | 0.61        | 0.74        | 0.69        | 0.63        | 0.69        |
| T5_NODE2VEC_TF-IDF_PCA | 0.51           | 0.80        | 0.72        | 0.70        | 0.67        | 0.66        | 0.68        |
| T5                     | 0.56           | 0.77        | 0.68        | 0.70        | 0.66        | 0.64        | 0.67        |
| T5_NODE2VEC            | 0.52           | 0.76        | 0.65        | 0.67        | 0.66        | 0.60        | 0.65        |
| NODE2VEC_TF-IDF_PCA    | 0.46           | 0.75        | 0.70        | 0.66        | 0.64        | 0.62        | 0.64        |
| NODE2VEC               | 0.40           | 0.60        | 0.45        | 0.54        | 0.50        | 0.42        | 0.48        |

|                  |             |             |             |             |             |             |             |
|------------------|-------------|-------------|-------------|-------------|-------------|-------------|-------------|
| Category Average | <b>0.64</b> | <b>0.79</b> | <b>0.67</b> | <b>0.72</b> | <b>0.71</b> | <b>0.67</b> | <b>0.70</b> |
|------------------|-------------|-------------|-------------|-------------|-------------|-------------|-------------|

(c)

|                        | GO-CC category |             |             |             |             |             |             |
|------------------------|----------------|-------------|-------------|-------------|-------------|-------------|-------------|
| Method names           | Low            | Middle      | High        | Specific    | Normal      | Shallow     | Method Mean |
| TF-IDF_PCA             | <b>0.84</b>    | <b>0.81</b> | 0.76        | <b>0.74</b> | <b>0.81</b> | <b>0.85</b> | <b>0.80</b> |
| MultiModalAE_768       | 0.76           | 0.78        | 0.74        | 0.69        | 0.78        | 0.80        | 0.76        |
| MultiModalAE_256       | 0.75           | 0.78        | 0.75        | 0.70        | 0.77        | 0.79        | 0.76        |
| MultiModalAE_1024      | 0.75           | 0.79        | 0.73        | 0.70        | 0.77        | 0.80        | 0.76        |
| SimpleAE_1024          | 0.74           | 0.79        | 0.74        | 0.69        | 0.77        | 0.79        | 0.75        |
| SimpleAE_768           | 0.74           | 0.79        | 0.73        | 0.69        | 0.77        | 0.78        | 0.75        |
| SimpleAE_512           | 0.74           | 0.78        | 0.73        | 0.69        | 0.76        | 0.79        | 0.75        |
| SimpleAE_256           | 0.72           | 0.78        | 0.75        | 0.67        | 0.75        | 0.80        | 0.74        |
| T5_TF-IDF_PCA          | 0.65           | 0.79        | <b>0.80</b> | 0.65        | 0.75        | 0.79        | 0.74        |
| TransferAE_768         | 0.69           | 0.76        | 0.70        | 0.66        | 0.71        | 0.76        | 0.71        |
| T5_NODE2VEC_TF-IDF_PCA | 0.62           | 0.76        | 0.78        | 0.63        | 0.71        | 0.77        | 0.71        |
| TransferAE_256         | 0.66           | 0.75        | 0.72        | 0.65        | 0.70        | 0.76        | 0.71        |
| TransferAE_1024        | 0.67           | 0.75        | 0.69        | 0.67        | 0.71        | 0.74        | 0.71        |
| TransferAE_512         | 0.65           | 0.76        | 0.70        | 0.63        | 0.70        | 0.76        | 0.70        |
| TS                     | 0.62           | 0.73        | 0.74        | 0.60        | 0.71        | 0.74        | 0.69        |
| T5_NODE2VEC            | 0.60           | 0.73        | 0.74        | 0.60        | 0.69        | 0.74        | 0.68        |
| NODE2VEC_TF-IDF_PCA    | 0.58           | 0.70        | 0.75        | 0.56        | 0.67        | 0.73        | 0.67        |
| NODE2VEC               | 0.47           | 0.61        | 0.60        | 0.50        | 0.55        | 0.60        | 0.55        |
| Category Average       | <b>0.68</b>    | <b>0.76</b> | <b>0.73</b> | <b>0.65</b> | <b>0.73</b> | <b>0.77</b> | <b>0.72</b> |

**Supplementary Table S3.** Positive predicted proteins by the fully connected neural network (FCNN) based immune escape protein prediction model.

| UniProt_ID | logFC    | FDR      | Gene_Name | NCBI ID | Ensemble ID     |
|------------|----------|----------|-----------|---------|-----------------|
| P01275     | 8,865552 | 4,02E-05 | GCG       | 2641    | ENSG00000115263 |
| P0DN86     | 7,741227 | 6,98E-13 | CGB5      | 93659   | ENSG00000189052 |
| P0DN86     | 7,206699 | 2,39E-14 | CGB5      | 93659   | ENSG00000189052 |
| Q7Z7D3     | 6,835872 | 4,58E-21 | VTCN1     | 79679   | ENSG00000134258 |
| Q7Z7D3     | 2,945165 | 1,46E-13 | VTCN1     | 79679   | ENSG00000134258 |
| Q96D42     | 6,369507 | 1,73E-25 | HAVCR1    | 26762   | ENSG00000113249 |
| O95715     | 4,441399 | 3,45E-22 | CXCL14    | 9547    | ENSG00000145824 |
| O14788     | 4,334118 | 3,13E-29 | TNFSF11   | 8600    | ENSG00000120659 |
| Q96CG8     | 3,929255 | 7,32E-58 | CTHRC1    | 115908  | ENSG00000164932 |
| Q9Y5U5     | 2,955532 | 7,00E-33 | TNFRSF18  | 8784    | ENSG00000186891 |
| P20809     | 2,943976 | 7,95E-22 | IL11      | 3589    | ENSG00000095752 |
| P17936     | 2,317512 | 2,09E-25 | IGFBP3    | 3486    | ENSG00000146674 |
| Q9BZS1     | 2,303428 | 1,02E-32 | FOXP3     | 50943   | ENSG00000049768 |
| Q13323     | 2,293214 | 2,13E-27 | BIK       | 638     | ENSG00000100290 |
| P19652     | 2,23785  | 2,77E-08 | ORM2      | 5005    | ENSG00000228278 |
| P13688     | 2,237467 | 1,12E-33 | CEACAM1   | 634     | ENSG00000079385 |
| O75509     | 2,12913  | 5,55E-50 | TNFRSF21  | 27242   | ENSG00000146072 |
| O95407     | 2,109516 | 3,38E-13 | TNFRSF6B  | 8771    | ENSG00000243509 |
| Q02223     | 2,00751  | 5,88E-14 | TNFRSF17  | 608     | ENSG00000048462 |
| Q01523     | 9,524979 | 1,27E-05 | DEFA5     | 1670    | ENSG00000285251 |
| P08833     | 4,580969 | 1,48E-10 | IGFBP1    | 3484    | ENSG00000146678 |
| P08254     | 4,565836 | 1,99E-21 | MMP3      | 4314    | ENSG00000149968 |
| P09238     | 4,253979 | 5,09E-17 | MMP10     | 4319    | ENSG00000166670 |
| P39900     | 4,224654 | 9,31E-28 | MMP12     | 4321    | ENSG00000262406 |
| P02760     | 4,024653 | 3,36E-13 | AMBP      | 259     | ENSG00000106927 |
| O14514     | 3,891797 | 9,72E-18 | ADGRB1    | 575     | ENSG00000181790 |
| Q8N6Q3     | 3,645404 | 1,93E-11 | CD177     | 57126   | ENSG00000204936 |
| P17787     | 3,227424 | 2,04E-11 | CHRNA2    | 1141    | ENSG00000160716 |
| Q9UKX5     | 3,171847 | 5,48E-31 | ITGA11    | 22801   | ENSG00000137809 |
| P52797     | 3,103647 | 2,87E-59 | EFNA3     | 1944    | ENSG00000143590 |
| Q5T4W7     | 3,030827 | 3,57E-24 | ARTN      | 9048    | ENSG00000117407 |
| Q96NY8     | 2,473901 | 4,52E-48 | NECTIN4   | 81607   | ENSG00000143217 |

|        |          |           |         |        |                 |
|--------|----------|-----------|---------|--------|-----------------|
| Q9UM44 | 2,40222  | 7,18E-07  | HHLA2   | 11148  | ENSG00000114455 |
| P01215 | 9,463754 | 2,21E-11  | CGA     | 1081   | ENSG00000135346 |
| Q9NPF7 | 2,845283 | 9,83E-27  | IL23A   | 51561  | ENSG00000110944 |
| O14944 | 2,666213 | 1,50E-08  | EREG    | 2069   | ENSG00000124882 |
| P14780 | 2,224398 | 1,03E-18  | MMP9    | 4318   | ENSG00000100985 |
| Q9HB29 | 2,925007 | 8,98E-38  | IL1RL2  | 8808   | ENSG00000115598 |
| P52798 | 2,354053 | 5,75E-72  | EFNA4   | 1945   | ENSG00000243364 |
| Q96LA5 | 2,21011  | 3,41E-14  | FCRL2   | 79368  | ENSG00000132704 |
| Q9H9P2 | 2,138284 | 1,36E-11  | CHODL   | 140578 | ENSG00000154645 |
| P00751 | 2,073484 | 4,33E-21  | CFB     | 629    | ENSG00000243649 |
| P20851 | 2,674623 | 2,99E-13  | C4BPB   | 725    | ENSG00000123843 |
| P55773 | 2,668675 | 3,04E-33  | CCL23   | 6368   | ENSG00000276114 |
| P55773 | -2,42499 | 4,53E-43  | CCL23   | 6368   | ENSG00000276114 |
| Q03167 | -2,5219  | 3,11E-80  | TGFBR3  | 7049   | ENSG00000069702 |
| Q9NPB9 | -2,39098 | 1,82E-52  | ACKR4   | 51554  | ENSG00000129048 |
| Q6UXG3 | -4,84461 | 1,04E-91  | CD300LG | 146894 | ENSG00000161649 |
| O43915 | -3,43457 | 1,50E-60  | VEGFD   | 2277   | ENSG00000165197 |
| P32241 | -3,25065 | 1,55E-119 | VIPR1   | 7433   | ENSG00000114812 |
| P25090 | -3,02174 | 3,40E-82  | FPR2    | 2358   | ENSG00000171049 |
| P16581 | -2,87073 | 8,04E-53  | SELE    | 6401   | ENSG00000007908 |
| P03951 | -2,75323 | 9,43E-22  | F11     | 2160   | ENSG00000088926 |
| Q8IWL2 | -2,67825 | 3,10E-28  | SFTPA1  | 653509 | ENSG00000122852 |
| P48740 | -2,67163 | 2,41E-59  | MASP1   | 5648   | ENSG00000127241 |
| Q9UQV4 | -2,6159  | 1,08E-67  | LAMP3   | 27074  | ENSG00000078081 |
| P37023 | -2,42638 | 1,05E-153 | ACVRL1  | 94     | ENSG00000139567 |
| Q16627 | -2,39853 | 4,68E-47  | CCL14   | 6358   | ENSG00000277236 |
| P23560 | -2,32663 | 5,80E-30  | BDNF    | 627    | ENSG00000176697 |
| P07204 | -2,31934 | 1,05E-84  | THBD    | 7056   | ENSG00000178726 |
| P22455 | -2,31935 | 4,16E-42  | FGFR4   | 2264   | ENSG00000160867 |
| P57087 | -2,3185  | 4,32E-112 | JAM2    | 58494  | ENSG00000154721 |
| Q13201 | -2,27087 | 9,79E-50  | MMRN1   | 22915  | ENSG00000138722 |
| P16109 | -2,22763 | 4,37E-57  | SELP    | 6403   | ENSG00000174175 |
| Q8NC01 | -2,19077 | 3,82E-98  | CLEC1A  | 51267  | ENSG00000150048 |
| Q9NPY3 | -2,09928 | 7,46E-90  | CD93    | 22918  | ENSG00000125810 |
| P19876 | -2,01612 | 2,06E-29  | CXCL3   | 2921   | ENSG00000163734 |

|        |          |           |         |        |                 |
|--------|----------|-----------|---------|--------|-----------------|
| Q01638 | -2,9452  | 5,62E-36  | IL1RL1  | 9173   | ENSG00000115602 |
| P25024 | -2,75025 | 8,12E-54  | CXCR1   | 3577   | ENSG00000163464 |
| Q93033 | -2,72256 | 2,46E-120 | CD101   | 9398   | ENSG00000134256 |
| P25025 | -2,50148 | 8,07E-61  | CXCR2   | 3579   | ENSG00000180871 |
| Q99075 | -2,45569 | 1,35E-83  | HBEGF   | 1839   | ENSG00000113070 |
| P19875 | -2,45376 | 1,52E-48  | CXCL2   | 2920   | ENSG00000081041 |
| P78380 | -2,39509 | 3,35E-60  | OLR1    | 4973   | ENSG00000173391 |
| Q9Y279 | -2,24521 | 1,16E-55  | VSIG4   | 11326  | ENSG00000155659 |
| P16671 | -2,77634 | 2,69E-64  | CD36    | 948    | ENSG00000135218 |
| Q8IWL1 | -2,55482 | 1,26E-25  | SFTPA2  | 729238 | ENSG00000185303 |
| Q9HD89 | 3,732392 | 5,73E-33  | RETN    | 56729  | ENSG00000104918 |
| Q9HD89 | 3,341803 | 2,35E-14  | RETN    | 56729  | ENSG00000104918 |
| Q9HD89 | -2,84057 | 1,89E-32  | RETN    | 56729  | ENSG00000104918 |
| Q15109 | -4,82561 | 3,21E-126 | AGER    | 177    | ENSG00000204305 |
| P22897 | -2,23222 | 1,20E-45  | MRC1    | 4360   | ENSG00000260314 |
| Q8IU80 | 2,640636 | 4,25E-12  | TMPRSS6 | 164656 | ENSG00000187045 |
| O76076 | -2,03246 | 1,97E-44  | CCN5    | 8839   | ENSG00000064205 |
| Q2I0M5 | -2,12972 | 6,21E-26  | RSPO4   | 343637 | ENSG00000101282 |
| P11686 | -4,50559 | 3,35E-60  | SFTPC   | 6440   | ENSG00000168484 |
| P09466 | 8,080022 | 1,50E-23  | PAEP    | 5047   | ENSG00000122133 |
| Q9NRS4 | 5,009729 | 2,27E-52  | TMPRSS4 | 56649  | ENSG00000137648 |
| P00749 | 2,730385 | 1,23E-26  | PLAU    | 5328   | ENSG00000122861 |
| Q92563 | -3,04369 | 7,78E-130 | SPOCK2  | 9806   | ENSG00000107742 |
| P30872 | 7,634012 | 9,02E-08  | SSTR1   | 6751   | ENSG00000139874 |
| P50052 | 3,237664 | 3,79E-17  | AGTR2   | 186    | ENSG00000180772 |
| P29323 | 2,488499 | 3,04E-30  | EPHB2   | 2048   | ENSG00000133216 |
| Q9H4F8 | 4,122351 | 1,24E-18  | SMOC1   | 64093  | ENSG00000198732 |
| Q6UX06 | 6,660903 | 5,00E-14  | OLFM4   | 10562  | ENSG00000102837 |
| O60894 | 2,371534 | 6,77E-25  | RAMP1   | 10267  | ENSG00000132329 |
| O60609 | 3,187024 | 3,20E-13  | GFRA3   | 2676   | ENSG00000146013 |
| Q14392 | -2,20163 | 2,78E-105 | LRRC32  | 2615   | ENSG00000137507 |
| P21453 | -2,7118  | 2,34E-165 | S1PR1   | 1901   | ENSG00000170989 |
| P24530 | -3,40121 | 4,34E-159 | EDNRB   | 1910   | ENSG00000136160 |
| A0PJX4 | 2,096675 | 2,02E-06  | SHISA3  | 152573 | ENSG00000178343 |
| Q08629 | 3,28676  | 5,32E-21  | SPOCK1  | 6695   | ENSG00000152377 |

|        |          |           |          |        |                 |
|--------|----------|-----------|----------|--------|-----------------|
| O94907 | 2,55148  | 3,23E-09  | DKK1     | 22943  | ENSG00000107984 |
| Q4LDE5 | -2,02701 | 1,64E-38  | SVEP1    | 79987  | ENSG00000165124 |
| Q9BU40 | -2,18048 | 1,54E-31  | CHRD1    | 91851  | ENSG00000101938 |
| O60896 | -3,05908 | 1,87E-175 | RAMP3    | 10268  | ENSG00000122679 |
| Q8IUB2 | 4,361843 | 3,41E-32  | WFDC3    | 149708 | ENSG00000175121 |
| Q16849 | 5,094703 | 1,46E-16  | PTPRN    | 5798   | ENSG00000054356 |
| Q7Z304 | -2,65006 | 4,70E-53  | MAMDC2   | 256691 | ENSG00000165072 |
| Q92832 | 3,537816 | 2,40E-07  | NELL1    | 4745   | ENSG00000165973 |
| Q01726 | 2,111151 | 8,60E-36  | MC1R     | 4157   | ENSG00000258839 |
| Q9Y5Y7 | -3,12108 | 9E-115    | LYVE1    | 10894  | ENSG00000133800 |
| A6NMZ7 | -2,80342 | 2,12E-52  | COL6A6   | 131873 | ENSG00000206384 |
| Q9UKZ9 | -2,26452 | 1,43E-32  | PCOLCE2  | 26577  | ENSG00000163710 |
| Q8TCV5 | 3,49637  | 2,15E-04  | WFDC5    | 149708 | ENSG00000175121 |
| P07550 | -2,96402 | 7,01E-112 | ADRB2    | 154    | ENSG00000169252 |
| P82987 | -2,27642 | 6,44E-13  | ADAMTSL3 | 57188  | ENSG00000156218 |
| P53708 | -2,32985 | 3,39E-54  | ITGA8    | 8516   | ENSG00000077943 |
| P08588 | -2,1072  | 1,09E-32  | ADRB1    | 153    | ENSG00000043591 |
| Q6UWQ7 | -2,97405 | 6,67E-58  | IGFL2    | 147920 | ENSG00000204866 |
| Q9UBU2 | -2,08493 | 1,98E-22  | DKK2     | 27123  | ENSG00000155011 |
| Q99795 | 4,172214 | 9,39E-24  | GPA33    | 10223  | ENSG00000143167 |
| Q96DR8 | -2,18789 | 1,08E-59  | MUCL1    | 118430 | ENSG00000172551 |
| Q969J5 | -2,61162 | 2,14E-29  | IL22RA2  | 116379 | ENSG00000164485 |
| Q8N6C5 | 3,935556 | 1,40E-07  | IGSF1    | 3547   | ENSG00000147255 |
| Q7Z408 | 4,0282   | 5,57E-26  | CSMD2    | 114784 | ENSG00000121904 |

**Supplementary Table S4.** Literature validated potential immune-escape therapy targets.

| UniProt_id | logFC            | FDR     | Gene_Name | NCBI ID | References                                                                                               |
|------------|------------------|---------|-----------|---------|----------------------------------------------------------------------------------------------------------|
| Q7Z7D3     | 2.94             | 1.5E-13 | VTCN1     | 79679   | doi://10.1016/j.cellimm.2019.104008<br>doi://10.1016/j.immuni.2018.03.018                                |
| Q96D42     | 6.37             | 1.7E-25 | HAVCR1    | 26762   | doi://10.1155/2016/8605134                                                                               |
| O95715     | 4.441            | 3.5E-22 | CXCL14    | 9547    | doi://10.3390/ijms20081872<br>doi://10.1038/srep09083                                                    |
| O14788     | 4.334            | 3.1E-29 | TNFSF11   | 8600    | doi://10.3390/ijms20092183                                                                               |
| Q96CG8     | 3.929            | 7.3E-58 | CTHRC1    | 115908  | doi://10.1155/2020/9578701<br>doi://10.3892/etm.2020.8833                                                |
| Q9Y5U5     | 2.956            | 7.0E-33 | TNFRSF18  | 8784    | doi://10.1186/s40425-017-0247-0<br>doi://10.4049/jimmunol.1001308<br>doi://10.1158/1078-0432.CCR-16-2000 |
| P20809     | 2.944            | 8.0E-22 | IL11      | 3589    | doi://10.1038/srep13650                                                                                  |
| P17936     | 2.318            | 2.1E-25 | IGFBP3    | 3486    | doi://10.1074/jbc.M110.122226                                                                            |
| Q9BZS1     | 2.303            | 1.0E-32 | FOXP3     | 50943   | doi://10.1038/cmi.2015.10                                                                                |
| Q13323     | 2.293            | 2.1E-27 | BIK       | 638     | doi://10.1038/s41467-017-00975-w<br>doi://10.3389/fphys.2017.00761<br>doi://10.1164/rccm.201011-1930OC   |
| P19652     | 2.238            | 2.8E-8  | ORM2      | 5005    | doi://10.1046/j.1365-2567.1996.d01-672.x<br>doi://10.3748/wjg.v26.i8.804                                 |
| P13688     | 2.238            | 1.1E-33 | CEACAM1   | 634     | doi://10.1084/jem.20102575                                                                               |
| O75509     | 2.129            | 5.6E-50 | TNFRSF21  | 27242   | doi://10.1007/s00262-007-0413-1                                                                          |
| O95407     | 2.11             | 3.4E-13 | TNFRSF6B  | 8771    | doi://10.1186/s12929-017-0347-7                                                                          |
| Q02223     | 2.008            | 5.9E-14 | TNFRSF17  | 608     | doi://10.1186/s13045-020-00962-7                                                                         |
| Q9NPF7     | 2.845            | 9.8E-27 | IL23A     | 51561   | doi://10.1007/s00262-006-0171-5                                                                          |
| O14944     | 2.666            | 1.5E-8  | EREG      | 2069    | doi://10.1016/j.semcd.2014.03.005                                                                        |
| P14780     | 2.224            | 1.0E-18 | MMP9      | 4318    | doi://10.1016/j.bbrc.2015.01.067                                                                         |
| Q03167     | -2.52190<br>3475 | 3.1E-80 | TGFBR3    | 7049    | doi://10.1158/0008-5472.CAN-06-3117<br>doi://10.1172/JCI29293<br>doi://10.1093/carcin/bgp271             |
| Q9NPB9     | -2.39098<br>1086 | 1.8E-52 | ACKR4     | 51554   | doi://10.1084/jem.20190634<br>doi://10.1007/s11033-016-3995-x<br>doi://10.3892/etm.2018.7007             |

**Supplementary Table S5.** Hyperparameter search space for the HOPE model.

| Hyperparameter name | Search Space                                                         |
|---------------------|----------------------------------------------------------------------|
| d (dimension)       | [10,50,100,200,500,1000]                                             |
| $\beta$ (beta)      | [0.00390625, 0.0078125, 0.015625, 0.03125, 0.0625, 0.125, 0.25, 0.5] |

**Supplementary Table S6.** Hyperparameter search space for the Node2Vec model.

| Hyperparameter name             | Search Space             |
|---------------------------------|--------------------------|
| d (dimension)                   | [10,50,100,200,500,1000] |
| max_iter (number of iterations) | [1]                      |
| walk_len                        | [80]                     |
| con_size (context window size)  | [80]                     |
| num_walks (number of walks)     | [10]                     |
| P (random walk parameter p)     | [ 0.25, 0.50,1, 2]       |
| Q (random walk parameter q)     | [ 0.25, 0.50,1, 2]       |

**Supplementary Table S7.** Performance results of the immune-escape protein prediction model (which utilises MultiModalAE model's representations as input feature vectors).

| <b>Classifier Name</b>                | <b>FC-NN (4 hidden layer 500 epochs)</b> |
|---------------------------------------|------------------------------------------|
| Accuracy                              | 0,87                                     |
| Accuracy Standard Deviation           | 0,01                                     |
| F1-Micro                              | 0,87                                     |
| F1-Micro Standard Deviation           | 0,05                                     |
| F1-Macro                              | 0,74                                     |
| F1-Macro Standard Deviation           | 0,06                                     |
| F-Maximum                             | 0,52                                     |
| F-Maximum Standard Deviation          | 0,13                                     |
| F1-Weighted                           | 0,86                                     |
| F1-Weighted Standard Deviation        | 0,04                                     |
| Precision Micro                       | 0,87                                     |
| Precision Micro Standard Deviation    | 0,05                                     |
| Precision Macro                       | 0,80                                     |
| Precision Macro Standard Deviation    | 0,11                                     |
| Precision Weighted                    | 0,87                                     |
| Precision_Weighted Standard Deviation | 0,05                                     |
| Recall Micro                          | 0,87                                     |
| Recall Micro Standard Deviation       | 0,05                                     |
| Recall Macro                          | 0,72                                     |
| Recall Macro Standard Deviation       | 0,05                                     |

|                                     |      |
|-------------------------------------|------|
| Recall Weighted                     | 0,87 |
| Recall Weighted Standard Deviation  | 0,05 |
| Hamming Distance                    | 0,13 |
| Hamming Distance Standard Deviation | 0,05 |
| AUC                                 | 0,72 |
| AUC Standard Deviation              | 0,05 |
| MCC                                 | 0,50 |

**Supplementary Table S8.** The number of proteins for each GO category in the dataset used in the protein function prediction benchmark (Unsal et al. 2022).

|                                                                                                       |          |    | Grouping GO terms in terms of<br>the number of annotations |        |     |
|-------------------------------------------------------------------------------------------------------|----------|----|------------------------------------------------------------|--------|-----|
|                                                                                                       |          |    | High                                                       | Middle | Low |
| Grouping GO terms considering the specificity of the term (i.e., location on the hierarchy of GO DAG) | Shallow  | BP | 3,386                                                      | 896    | 27  |
|                                                                                                       |          | MF | 3,039                                                      | 613    | 41  |
|                                                                                                       |          | CC | 7,186                                                      | 413    | 55  |
|                                                                                                       | Normal   | BP | 3,288                                                      | 452    | 28  |
|                                                                                                       |          | MF | 1,324                                                      | 369    | 31  |
|                                                                                                       |          | CC | 6,478                                                      | 562    | 47  |
|                                                                                                       | Specific | BP | 2,025                                                      | 623    | 42  |
|                                                                                                       |          | MF | 0                                                          | 204    | 41  |
|                                                                                                       |          | CC | 0                                                          | 413    | 54  |

**Supplementary Table S9.** Identifiers of GO terms that are incorporated into each of the 25 different multi-task models constructed for the protein function prediction benchmark(Unsal et al. 2022).

|                                                                                                       |          |    | Grouping GO terms in terms of the number of annotations            |                                                                    |                                                                    |
|-------------------------------------------------------------------------------------------------------|----------|----|--------------------------------------------------------------------|--------------------------------------------------------------------|--------------------------------------------------------------------|
|                                                                                                       |          |    | High                                                               | Middle                                                             | Low                                                                |
| Grouping GO terms considering the specificity of the term (i.e., location on the hierarchy of GO DAG) | Shallow  | BP | GO:0007399<br>GO:0006259<br>GO:0007167<br>GO:0006886<br>GO:0051707 | GO:0043488<br>GO:0043312<br>GO:0038096<br>GO:0006637<br>GO:0051091 | GO:0032933<br>GO:0006348<br>GO:0042989<br>GO:0000054<br>GO:0039529 |
|                                                                                                       |          | MF | GO:0016818<br>GO:0022890<br>GO:0046872<br>GO:0004672<br>GO:0000981 | GO:0036459<br>GO:0046943<br>GO:0005524<br>GO:0005244<br>GO:0022835 | GO:0015187<br>GO:0008568<br>GO:0008508<br>GO:0005328<br>GO:0043138 |
|                                                                                                       |          | CC | GO:0005789<br>GO:1990234<br>GO:1903561<br>GO:0005740<br>GO:0070013 | GO:0008076<br>GO:0005762<br>GO:0005747<br>GO:0036464<br>GO:0044853 | GO:0000124<br>GO:0097165<br>GO:0008024<br>GO:0032590<br>GO:0033162 |
|                                                                                                       | Normal   | BP | GO:0070647<br>GO:0016071<br>GO:0015833<br>GO:0048699<br>GO:0019752 | GO:0071427<br>GO:0016573<br>GO:0006613<br>GO:0031146<br>GO:0051092 | GO:0098703<br>GO:0061740<br>GO:0014808<br>GO:0000056<br>GO:0050482 |
|                                                                                                       |          | MF | GO:0016462<br>GO:0044212                                           | GO:0003774<br>GO:0008227<br>GO:0004866<br>GO:0004714<br>GO:0004843 | GO:0016934<br>GO:0022848<br>GO:0005314<br>GO:0003689<br>GO:0005335 |
|                                                                                                       |          | CC | GO:0070062<br>GO:0000228<br>GO:0031981<br>GO:0015630<br>GO:0005768 | GO:0000502<br>GO:0005925<br>GO:0022627<br>GO:0030665<br>GO:0034705 | GO:0036020<br>GO:0070081<br>GO:0044754<br>GO:1990454<br>GO:0031089 |
|                                                                                                       | Specific | BP | GO:0045944<br>GO:0001934<br>GO:1903507                             | GO:1903169<br>GO:0050773<br>GO:0071805<br>GO:0031124<br>GO:0000209 | GO:0043984<br>GO:0034625<br>GO:0006231<br>GO:0046323<br>GO:0072539 |
|                                                                                                       |          | MF | -                                                                  | GO:0061733<br>GO:0003777<br>GO:0004386                             | GO:0004957<br>GO:0008511<br>GO:0004571<br>GO:0017049<br>GO:0097199 |
|                                                                                                       |          | CC | -                                                                  | GO:0005766<br>GO:0016591<br>GO:0101002<br>GO:0008021               | GO:0019908<br>GO:0005767<br>GO:0032009<br>GO:0005736<br>GO:0099061 |

**Supplementary Table S10.** Overall performance results in ontology-based protein function prediction benchmark for GO: (a) molecular function, (b) biological process, (c) cellular component(Unsal et al. 2022).

(a)

| Methods           | Accuracy    | F1-Weighted | Precision   | Recall      | Hamming     |
|-------------------|-------------|-------------|-------------|-------------|-------------|
| InterPro2GO       | 0.28        | 0.37        | 0.86        | 0.28        | 0.20        |
| UniRule2GO        | 0.01        | 0.01        | 0.54        | 0.01        | 0.27        |
| Ensembl-Orthology | 0.11        | 0.20        | 0.89        | 0.12        | 0.24        |
| BLAST             | 0.84        | 0.87        | 0.92        | 0.86        | 0.05        |
| HMMER             | <b>0.86</b> | 0.89        | 0.91        | <b>0.89</b> | 0.05        |
| K-Sep             | 0.71        | 0.81        | 0.85        | 0.81        | 0.09        |
| APAAC             | 0.47        | 0.58        | 0.67        | 0.60        | 0.17        |
| PFAM              | 0.81        | 0.86        | <b>0.93</b> | 0.84        | 0.06        |
| AAC               | 0.39        | 0.41        | 0.49        | 0.44        | 0.20        |
| ProtVec           | 0.52        | 0.64        | 0.68        | 0.67        | 0.17        |
| Gene2Vec          | 0.44        | 0.53        | 0.59        | 0.53        | 0.20        |
| Learned-Vec       | 0.59        | 0.68        | 0.72        | 0.68        | 0.14        |
| Mut2Vec           | 0.49        | 0.57        | 0.63        | 0.57        | 0.18        |
| TCGA-Embedding    | 0.30        | 0.34        | 0.41        | 0.36        | 0.26        |
| SeqVec            | 0.84        | 0.89        | 0.91        | 0.88        | 0.05        |
| MSA-Transformer   | 0.59        | 0.67        | 0.73        | 0.68        | 0.14        |
| CPCProt           | 0.52        | 0.65        | 0.70        | 0.68        | 0.16        |
| ProtBERT-BFD      | 0.77        | 0.85        | 0.87        | 0.84        | 0.07        |
| TAPE-BERT-PFAM    | 0.78        | 0.85        | 0.86        | 0.85        | 0.07        |
| ESM-1b            | 0.77        | 0.83        | 0.87        | 0.84        | 0.07        |
| ProtALBERT        | 0.83        | 0.89        | 0.91        | 0.87        | 0.05        |
| ProtXLNet         | 0.71        | 0.82        | 0.85        | 0.82        | 0.09        |
| UniRep            | 0.75        | 0.82        | 0.86        | 0.82        | 0.08        |
| ProtT5-XL         | <b>0.86</b> | <b>0.90</b> | 0.92        | <b>0.89</b> | <b>0.04</b> |

(b)

| Methods           | Accuracy    | F1-Weighted | Precision   | Recall      | Hamming     |
|-------------------|-------------|-------------|-------------|-------------|-------------|
| InterPro2GO       | 0.07        | 0.11        | 0.50        | 0.07        | 0.20        |
| UniRule2GO        | 0.01        | 0.01        | 0.19        | 0.01        | 0.21        |
| Ensembl-Orthology | 0.15        | 0.24        | <b>0.72</b> | 0.16        | 0.18        |
| BLAST             | 0.46        | 0.56        | 0.68        | 0.50        | 0.15        |
| HMMER             | 0.50        | 0.61        | 0.64        | 0.60        | 0.16        |
| K-Sep             | 0.36        | 0.52        | 0.59        | 0.55        | 0.23        |
| APAAC             | 0.22        | 0.34        | 0.42        | 0.41        | 0.28        |
| PFAM              | 0.48        | 0.56        | 0.67        | 0.52        | 0.16        |
| AAC               | 0.16        | 0.19        | 0.32        | 0.20        | 0.25        |
| ProtVec           | 0.24        | 0.36        | 0.41        | 0.42        | 0.27        |
| Gene2Vec          | 0.31        | 0.44        | 0.49        | 0.42        | 0.23        |
| Learned-Vec       | 0.31        | 0.39        | 0.48        | 0.39        | 0.22        |
| Mut2Vec           | 0.33        | 0.43        | 0.49        | 0.42        | 0.22        |
| TCGA-Embedding    | 0.24        | 0.32        | 0.42        | 0.32        | 0.24        |
| SeqVec            | 0.50        | 0.60        | 0.65        | 0.59        | 0.16        |
| MSA-Transformer   | 0.32        | 0.47        | 0.57        | 0.52        | 0.23        |
| CPCProt           | 0.27        | 0.40        | 0.51        | 0.41        | 0.25        |
| ProtBERT-BFD      | 0.49        | 0.61        | 0.70        | 0.59        | 0.16        |
| TAPE-BERT-PFAM    | 0.40        | 0.54        | 0.61        | 0.55        | 0.20        |
| ESM-1b            | 0.42        | 0.53        | 0.64        | 0.55        | 0.19        |
| ProtALBERT        | 0.51        | 0.63        | 0.71        | 0.60        | 0.15        |
| ProtXLNet         | 0.37        | 0.50        | 0.61        | 0.51        | 0.20        |
| UniRep            | 0.38        | 0.48        | 0.60        | 0.49        | 0.21        |
| ProtT5-XL         | <b>0.57</b> | <b>0.66</b> | 0.71        | <b>0.63</b> | <b>0.13</b> |

(c)

| Methods           | Accuracy    | F1-Weighted | Precision   | Recall      | Hamming     |
|-------------------|-------------|-------------|-------------|-------------|-------------|
| InterPro2GO       | 0.22        | 0.27        | 0.72        | 0.22        | 0.18        |
| UniRule2GO        | 0.03        | 0.04        | 0.17        | 0.03        | 0.22        |
| Ensembl-Orthology | 0.16        | 0.26        | 0.72        | 0.17        | 0.19        |
| BLAST             | 0.49        | 0.57        | 0.70        | 0.53        | 0.14        |
| HMMER             | 0.49        | 0.60        | 0.65        | 0.59        | 0.16        |
| K-Sep             | 0.34        | 0.50        | 0.58        | 0.54        | 0.21        |
| APAAC             | 0.24        | 0.40        | 0.45        | 0.46        | 0.26        |
| PFAM              | 0.50        | 0.58        | 0.71        | 0.54        | 0.13        |
| AAC               | 0.24        | 0.23        | 0.28        | 0.28        | 0.23        |
| ProtVec           | 0.24        | 0.38        | 0.45        | 0.42        | 0.26        |
| Gene2Vec          | 0.37        | 0.50        | 0.55        | 0.50        | 0.19        |
| Learned-Vec       | 0.32        | 0.41        | 0.47        | 0.42        | 0.21        |
| Mut2Vec           | 0.36        | 0.46        | 0.53        | 0.46        | 0.19        |
| TCGA-Embedding    | 0.34        | 0.41        | 0.50        | 0.44        | 0.21        |
| SeqVec            | 0.50        | 0.61        | 0.68        | 0.59        | 0.15        |
| MSA-Transformer   | 0.34        | 0.50        | 0.59        | 0.52        | 0.21        |
| CPCProt           | 0.32        | 0.44        | 0.52        | 0.46        | 0.21        |
| ProtBERT-BFD      | 0.51        | 0.62        | 0.69        | 0.62        | 0.15        |
| TAPE-BERT-PFAM    | 0.45        | 0.58        | 0.66        | 0.58        | 0.17        |
| ESM-1b            | 0.47        | 0.61        | 0.70        | 0.63        | 0.16        |
| ProtALBERT        | 0.51        | 0.64        | 0.73        | 0.61        | 0.14        |
| ProtXLNet         | 0.45        | 0.59        | 0.67        | 0.60        | 0.17        |
| UniRep            | 0.38        | 0.53        | 0.59        | 0.57        | 0.19        |
| ProtT5-XL         | <b>0.59</b> | <b>0.68</b> | <b>0.76</b> | <b>0.66</b> | <b>0.12</b> |

**Supplementary Table S11.** The curated positive training dataset of the immune escape protein function prediction model.

| Protein_id | Gen_name | Protein names                                           |
|------------|----------|---------------------------------------------------------|
| O00559     | EBAG9    | Receptor-binding cancer antigen expressed on SiSo cells |
| O14920     | IKBKB    | Inhibitor of nuclear factor kappa-B kinase subunit beta |
| O95407     | TNFRSF6B | Tumor necrosis factor receptor superfamily member 6B    |
| P01137     | TGFB1    | Transforming growth factor beta-1 proprotein            |
| P01579     | IFNG     | Interferon gamma                                        |
| P05089     | ARG1     | Arginase-1                                              |
| P05362     | ICAM1    | Intercellular adhesion molecule 1                       |
| P14902     | IDO1     | Indoleamine 2,3-dioxygenase 1                           |
| P15692     | VEGFA    | Vascular endothelial growth factor A                    |
| P16070     | CD44     | CD44 antigen                                            |
| P16410     | CTLA4    | Cytotoxic T-lymphocyte protein 4                        |
| P17693     | HLA-G    | HLA class I histocompatibility antigen                  |
| P22301     | IL10     | Interleukin-10                                          |
| P25024     | CXCR1    | C-X-C chemokine receptor type 1                         |
| P25025     | CXCR2    | C-X-C chemokine receptor type 2                         |
| P28062     | PSMB8    | Proteasome subunit beta type-8                          |
| P29459     | IL12A    | Interleukin-12 subunit alpha                            |
| P33681     | CD80     | T-lymphocyte activation antigen CD80                    |
| P42081     | CD86     | T-lymphocyte activation antigen CD86                    |
| P48023     | FASLG    | Tumor necrosis factor ligand superfamily member 6       |
| P49913     | CAMP     | Cathelicidin antimicrobial peptide                      |
| P60568     | IL2      | Interleukin-2                                           |
| Q03518     | TAP1     | Antigen peptide transporter 1                           |
| Q08722     | CD47     | Leukocyte surface antigen CD47                          |
| Q9BZS1     | FOXP3    | Forkhead box protein P3                                 |
| Q9NZQ7     | CD274    | Programmed cell death 1 ligand 1                        |

**Supplementary Table S12.** The curated negative training dataset of the immune escape protein function prediction model.

| Uniprot_accession | Gen_name  | Protein names                                    |
|-------------------|-----------|--------------------------------------------------|
| O00519            | FAAH      | Fatty-acid amide hydrolase 1                     |
| O15091            | PRORP     | Mitochondrial ribonuclease P catalytic subunit   |
| O60939            | SCN2B     | Sodium channel subunit beta-2                    |
| O75127            | PTCD1     | Pentatricopeptide repeat-containing protein 1    |
| O75154            | RAB11FIP3 | Rab11 family-interacting protein 3               |
| O76070            | SNCG      | Gamma-synuclein                                  |
| O94817            | ATG12     | Ubiquitin-like protein ATG12                     |
| O95214            | LEPROTL1  | Leptin receptor overlapping transcript-like 1    |
| O95870            | ABHD16A   | Phosphatidylserine lipase ABHD16A                |
| P04201            | MAS1      | Proto-oncogene Mas                               |
| P04746            | AMY2A     | Pancreatic alpha-amylase                         |
| P07101            | TH        | Tyrosine 3-monooxygenase                         |
| P09131            | SLC10A3   | P3 protein                                       |
| P17098            | ZNF8      | Zinc finger protein 8                            |
| P21506            | ZNF10     | Zinc finger protein 10                           |
| P22033            | MMUT      | Methylmalonyl-CoA mutase                         |
| P22531            | SPRR2E    | Small proline-rich protein 2E                    |
| P22830            | FECH      | Ferrochelatase, mitochondrial                    |
| P23763            | VAMP1     | Vesicle-associated membrane protein 1            |
| P27144            | AK4       | Adenylate kinase 4                               |
| P33316            | DUT       | Deoxyuridine 5'-triphosphate nucleotidohydrolase |
| P35749            | MYH11     | Myosin-11                                        |
| P36776            | LONP1     | Lon protease homolog                             |
| P40123            | CAP2      | Adenylyl cyclase-associated protein 2            |
| P40425            | PBX2      | Pre-B-cell leukemia transcription factor 2       |
| P46059            | SLC15A1   | Solute carrier family 15 member 1                |
| P47775            | GPR12     | G-protein coupled receptor 12                    |
| P49419            | ALDH7A1   | Alpha-aminoadipic semialdehyde dehydrogenase     |
| P98179            | RBM3      | RNA-binding protein 3                            |
| Q01449            | MYL7      | Myosin regulatory light chain 2                  |
| Q01780            | EXOSC10   | Exosome complex component 10                     |
| Q04727            | TLE4      | Transducin-like enhancer protein 4               |
| Q05923            | DUSP2     | Dual specificity protein phosphatase 2           |

|        |          |                                                          |
|--------|----------|----------------------------------------------------------|
| Q0D2K0 | NIPAL4   | Magnesium transporter NIPA4                              |
| Q12874 | SF3A3    | Splicing factor 3A subunit 3                             |
| Q13472 | TOP3A    | DNA topoisomerase 3-alpha                                |
| Q13702 | RAPSN    | 43 kDa receptor-associated protein of the synapse        |
| Q14032 | BAAT     | Bile acid-CoA:amino acid N-acyltransferase               |
| Q14416 | GRM2     | Metabotropic glutamate receptor 2                        |
| Q14BN4 | SLMAP    | Sarcolemmal membrane-associated protein                  |
| Q15849 | SLC14A2  | Urea transporter 2                                       |
| Q49A26 | GLYR1    | Cytokine-like nuclear factor N-PAC                       |
| Q5C9Z4 | NOM1     | Nucleolar MIF4G domain-containing protein 1              |
| Q5SQQ9 | VAX1     | Ventral anterior homeobox 1                              |
| Q5T0N5 | FNBP1L   | Formin-binding protein 1-like                            |
| Q5TC63 | GRTP1    | Growth hormone-regulated TBC protein 1                   |
| Q5VW38 | GPR107   | Protein GPR107                                           |
| Q6E0U4 | DMKN     | Dermokine                                                |
| Q6ZU35 | CRACD    | Capping protein-inhibiting regulator of actin dynamics   |
| Q7Z3Z4 | PIWIL4   | Piwi-like protein 4                                      |
| Q86SZ2 | TRAPPC6B | Trafficking protein particle complex subunit 6B          |
| Q8IUZ0 | LRRC49   | Leucine-rich repeat-containing protein 49                |
| Q8IV01 | SYT12    | Synaptotagmin-12                                         |
| Q8IVS8 | GLYCK    | Glycerate kinase                                         |
| Q8IWS0 | PHF6     | PHD finger protein 6                                     |
| Q8N0X2 | SPAG16   | Sperm-associated antigen 16 protein                      |
| Q8N126 | CADM3    | Cell adhesion molecule 3                                 |
| Q8N142 | ADSS1    | Adenylosuccinate synthetase isozyme 1                    |
| Q8N841 | TTLL6    | Tubulin polyglutamylase TTLL6                            |
| Q8NB12 | SMYD1    | Histone-lysine N-methyltransferase SMYD1                 |
| Q8NBQ5 | HSD17B11 | Estradiol 17-beta-dehydrogenase 11                       |
| Q8NEM2 | SHCBP1   | SHC SH2 domain-binding protein 1                         |
| Q8NEV4 | MYO3A    | Myosin-IIIa                                              |
| Q8NHY3 | GAS2L2   | GAS2-like protein 2                                      |
| Q8NHY5 | HUS1B    | Checkpoint protein HUS1B                                 |
| Q8NI37 | PPTC7    | Protein phosphatase PTC7 homolog                         |
| Q8TB36 | GDAP1    | Ganglioside-induced differentiation-associated protein 1 |
| Q8TDJ6 | DMXL2    | DmX-like protein 2                                       |
| Q8TDY2 | RB1CC1   | RB1-inducible coiled-coil protein 1                      |

|        |         |                                                    |
|--------|---------|----------------------------------------------------|
| Q8TE73 | DNAH5   | Dynein axonemal heavy chain 5                      |
| Q8TEA1 | NSUN6   | tRNA (cytosine(72)-C(5))-methyltransferase NSUN6   |
| Q8WUY3 | PRUNE2  | Protein prune homolog 2                            |
| Q92502 | STARD8  | StAR-related lipid transfer protein 8              |
| Q92979 | EMG1    | Ribosomal RNA small subunit methyltransferase NEP1 |
| Q96A32 | MYL11   | Myosin regulatory light chain 11                   |
| Q96DA2 | RAB39B  | Ras-related protein Rab-39B                        |
| Q96ED9 | HOOK2   | Protein Hook homolog 2                             |
| Q96II8 | LRCH3   | DISP complex protein LRCH3                         |
| Q96K21 | ZFYVE19 | Abscission/NoCut checkpoint regulator              |
| Q96MY7 | FAM161B | Protein FAM161B                                    |
| Q96QS3 | ARX     | Homeobox protein ARX                               |
| Q96ST2 | IWS1    | Protein IWS1 homolog                               |
| Q99619 | SPSB2   | SPRY domain-containing SOCS box protein 2          |
| Q9BQI0 | AIF1L   | Allograft inflammatory factor 1-like               |
| Q9BRX5 | GIN53   | DNA replication complex GINS protein PSF3          |
| Q9BVG9 | PTDSS2  | Phosphatidylserine synthase 2                      |
| Q9BWD1 | ACAT2   | Acetyl-CoA acetyltransferase                       |
| Q9BXF9 | TEKT3   | Tektin-3                                           |
| Q9BXS4 | TMEM59  | Transmembrane protein 59                           |
| Q9BY50 | SEC11C  | Signal peptidase complex catalytic subunit SEC11C  |
| Q9BZV2 | SLC19A3 | Thiamine transporter 2                             |
| Q9C0A0 | CNTNAP4 | Contactin-associated protein-like 4                |
| Q9H1H9 | KIF13A  | Kinesin-like protein KIF13A                        |
| Q9H3H1 | TRIT1   | tRNA dimethylallyltransferase                      |
| Q9H8Y8 | GORASP2 | Golgi reassembly-stacking protein 2                |
| Q9HA82 | CERS4   | Ceramide synthase 4                                |
| Q9HB15 | KCNK12  | Potassium channel subfamily K member 12            |
| Q9HBJ0 | PLAC1   | Placenta-specific protein 1                        |
| Q9HC07 | TMEM165 | Putative divalent cation/proton antiporter TMEM165 |
| Q9HCH0 | NCKAP5L | Nck-associated protein 5-like                      |
| Q9NSB8 | HOMER2  | Homer protein homolog 2                            |
| Q9NUH8 | TMEM14B | Transmembrane protein 14B                          |
| Q9NUQ3 | TXLNG   | Gamma-taxilin                                      |
| Q9NVR5 | DNAAF2  | Protein kintoun                                    |

|        |         |                                                               |
|--------|---------|---------------------------------------------------------------|
| Q9NXX6 | NSMCE4A | Non-structural maintenance of chromosomes element 4 homolog A |
| Q9NZM3 | ITSN2   | Intersectin-2                                                 |
| Q9P013 | CWC15   | Spliceosome-associated protein CWC15 homolog                  |
| Q9P0P0 | RNF181  | E3 ubiquitin-protein ligase RNF181                            |
| Q9P2G1 | ANKIB1  | Ankyrin repeat and IBR domain-containing protein 1            |
| Q9P2N7 | KLHL13  | Kelch-like protein 13                                         |
| Q9UBH6 | XPR1    | Solute carrier family 53 member 1                             |
| Q9UBM4 | OPTC    | Opticin                                                       |
| Q9UBQ6 | EXTL2   | Exostosin-like 2                                              |
| Q9UHN6 | CEMIP2  | Inactive cell surface hyaluronidase CEMIP2                    |
| Q9Y227 | ENTPD4  | Ectonucleoside triphosphate diphosphohydrolase 4              |
| Q9Y283 | INVS    | Inversin                                                      |
| Q9Y2D0 | CA5B    | Carbonic anhydrase 5B                                         |
| Q9Y2D4 | EXOC6B  | Exocyst complex component 6B                                  |
| Q9Y2T2 | AP3M1   | AP-3 complex subunit mu-1                                     |
| Q9Y3M9 | ZNF337  | Zinc finger protein 337                                       |
| Q9Y473 | ZNF175  | Zinc finger protein 175                                       |
| Q9Y5Y0 | FLVCR1  | Heme transporter FLVCR1                                       |
| Q9Y6A4 | CFAP20  | Cilia- and flagella-associated protein 20                     |
| Q9Y6N5 | SQOR    | Sulfide:quinone oxidoreductase                                |

**Figure S1.1.** Protein representations of TF-IDF\_PCA for the nine GO groups belong to molecular function ([low, middle, high] x [shallow, normal, specific]). (a) MF High Normal (b) MF High Shallow (c) MF Low Normal (d) MF Low Shallow (e) MF Low Specific (f) MF Middle Shallow (g) MF Middle Specific.

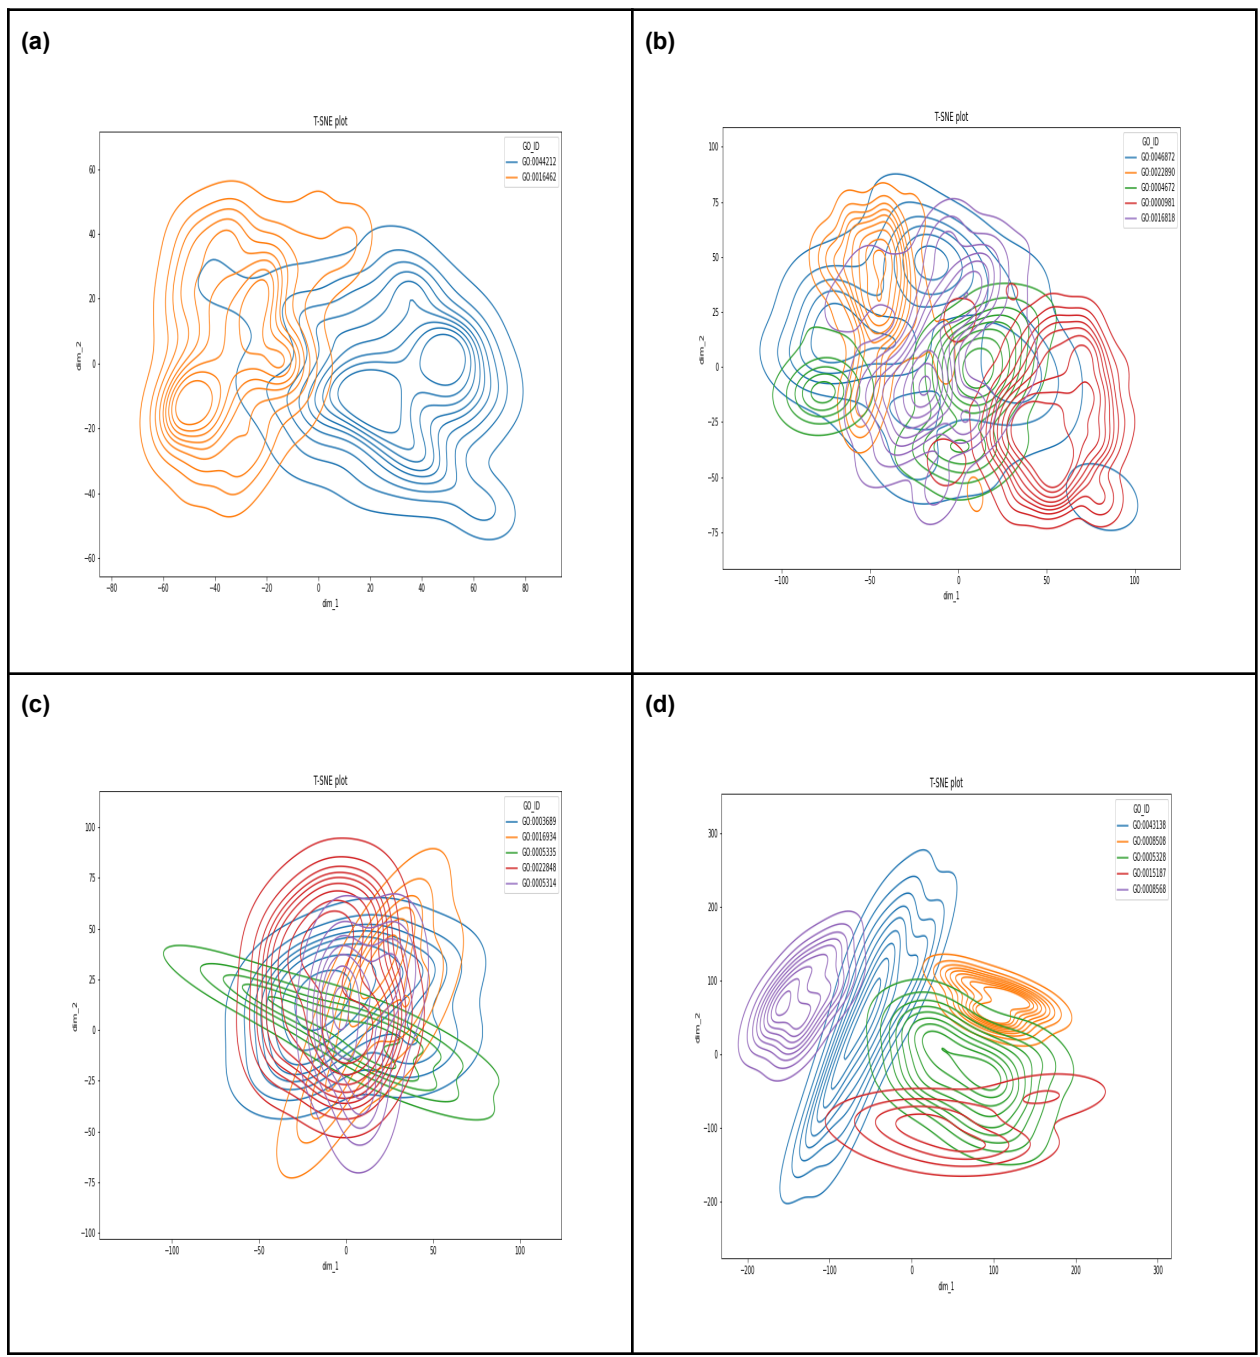

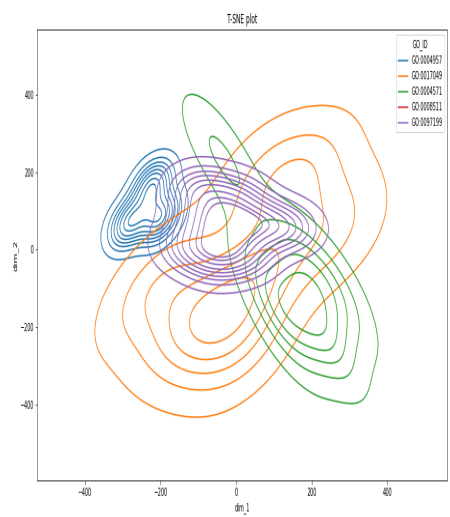

(e)

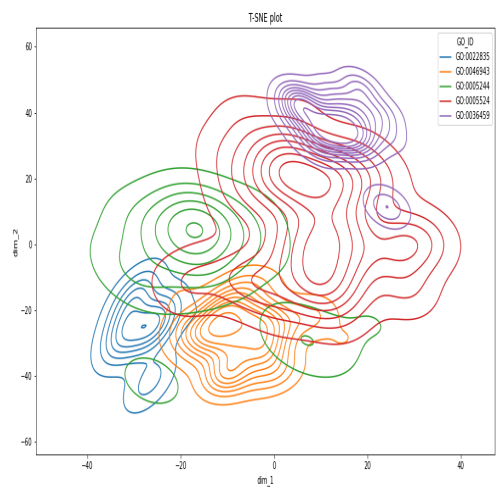

(f)

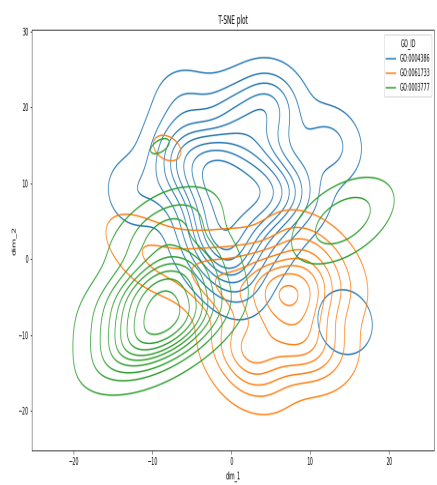

(g)

**Figure S1.2** T-SNE figures of protein representations of TF-IDF\_PCA for the nine GO groups belong to the biological process (BP) ([low, middle, high] x [shallow, normal, specific]). (a) BP High Normal (b) BP High Shallow (c) BP High Specific (d) BP Low Normal (e) BP Low Shallow (f) BP Low Specific (g) BP Middle Normal (h) BP Middle Specific (i) BP Middle Shallow.

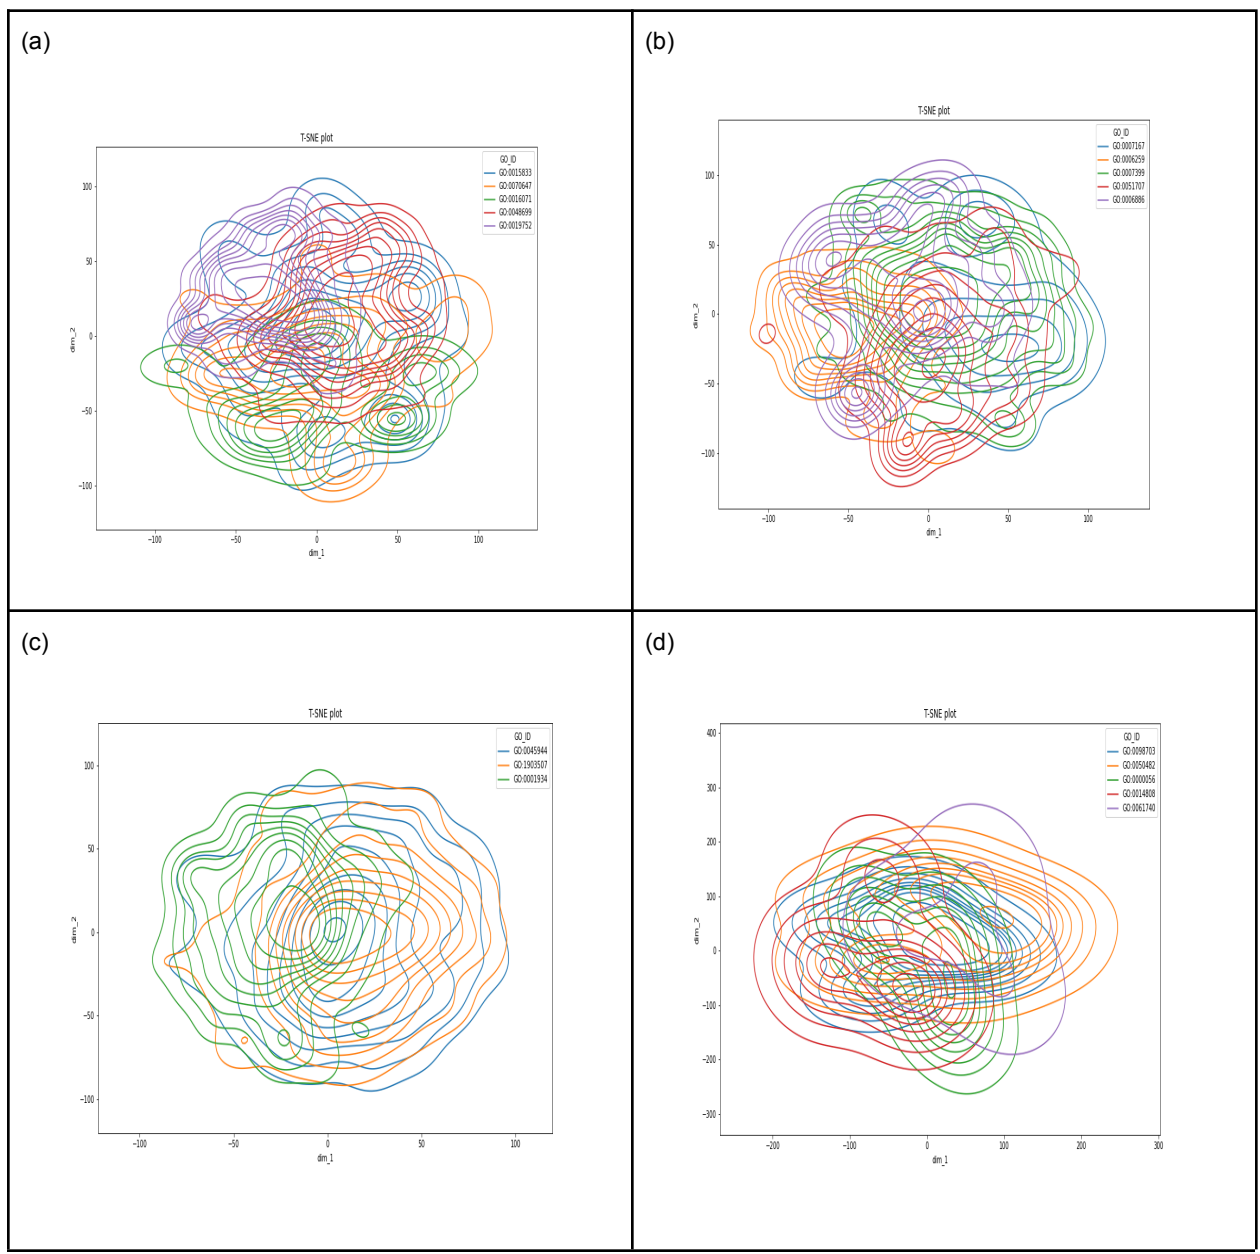

(e)

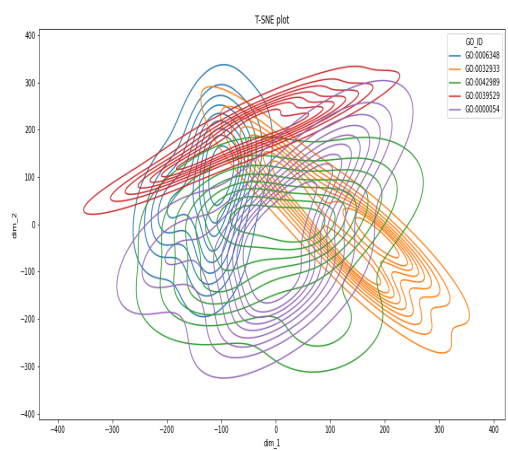

(f)

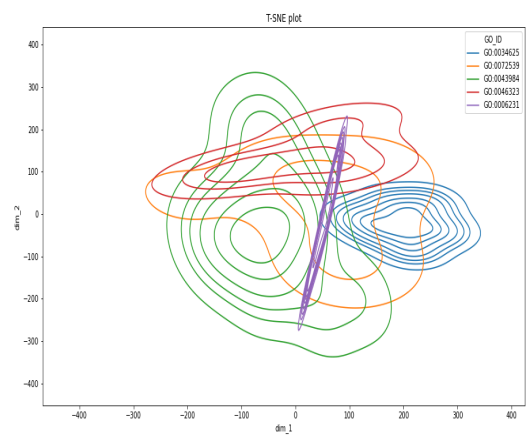

(g)

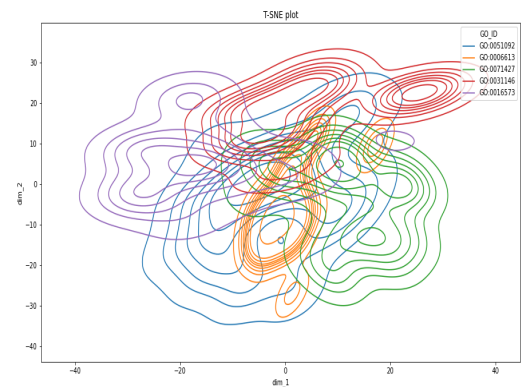

(h)

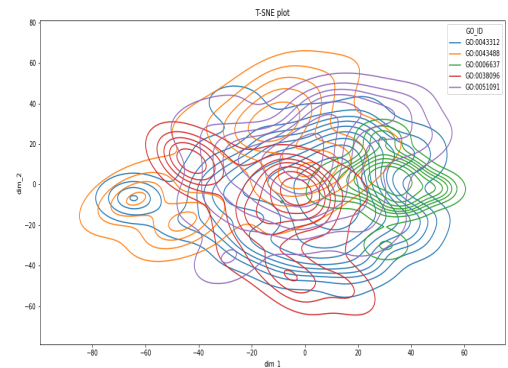

(i)

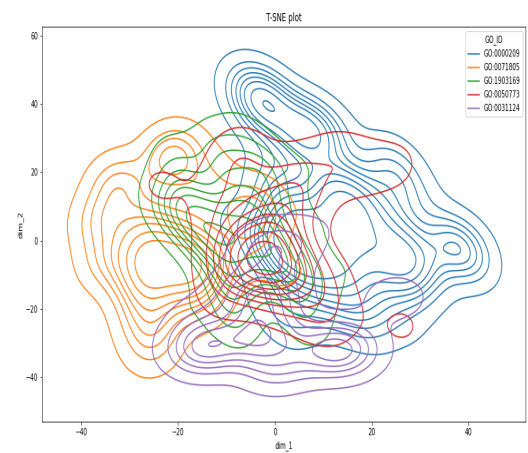

Fig

**Figure S1.3.** T-SNE figures of protein representations of TF-IDF\_PCA for the nine GO groups belong to the cellular component (CC) ([low, middle, high] x [shallow, normal, specific]). (a) CC High Normal (b) CC High Shallow (c) CC Low Normal (d) CC Low Shallow (e) CC Low Specific (f) CC Middle Normal (g) CC Middle Shallow (h) CC Middle Specific.

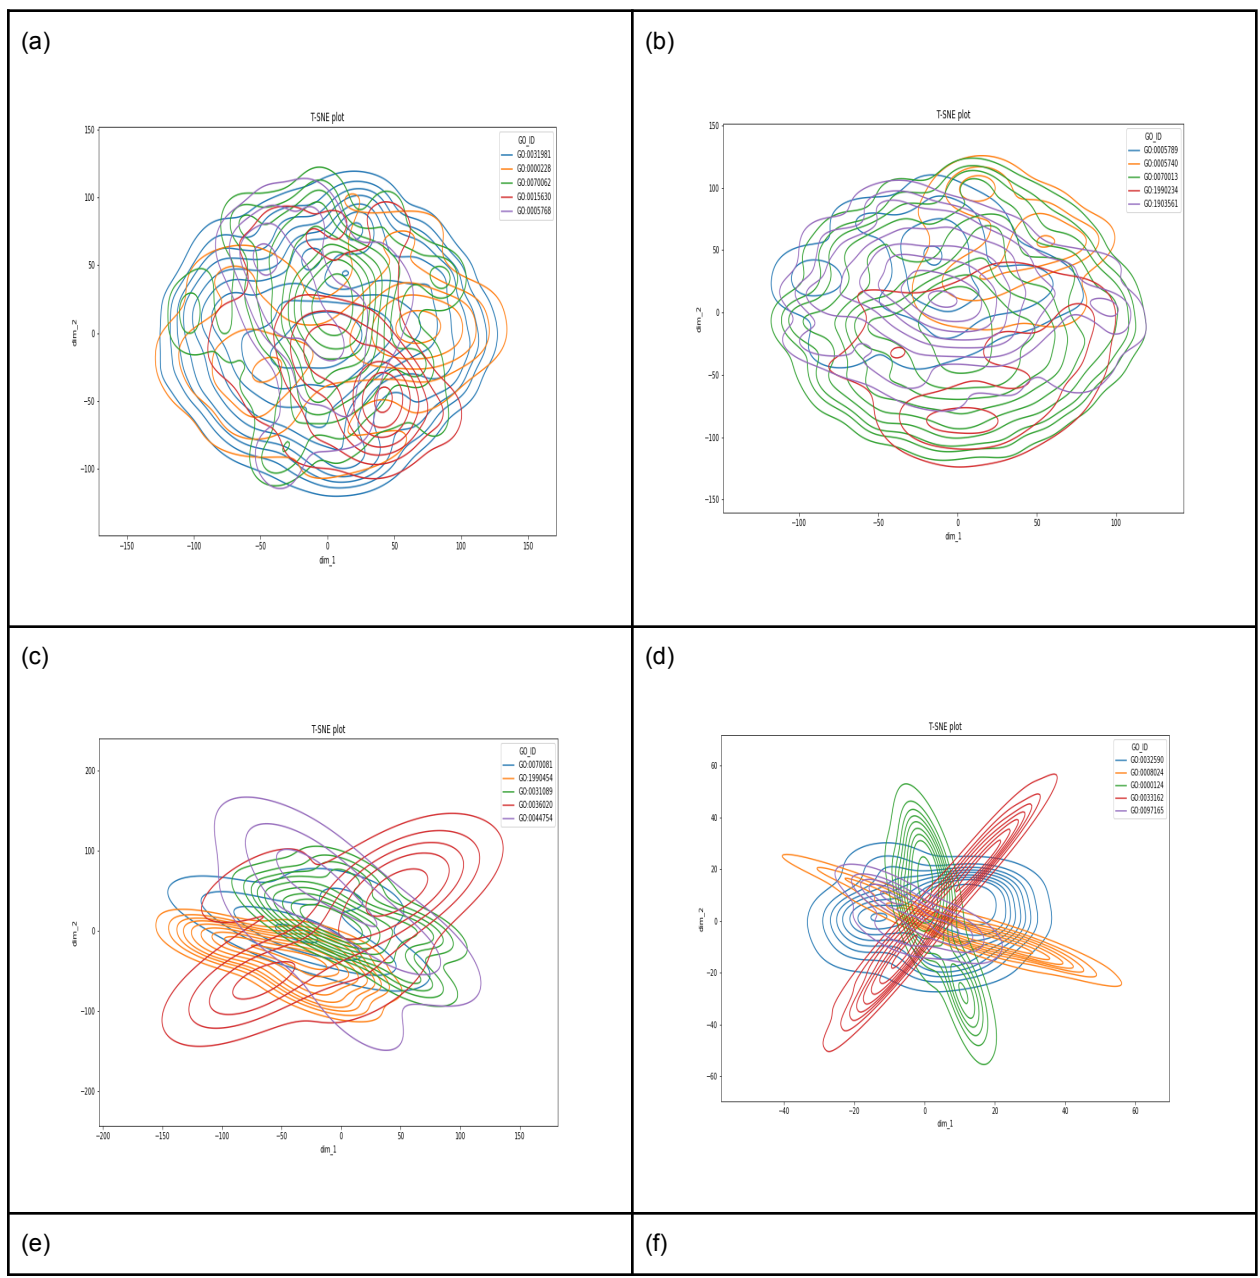

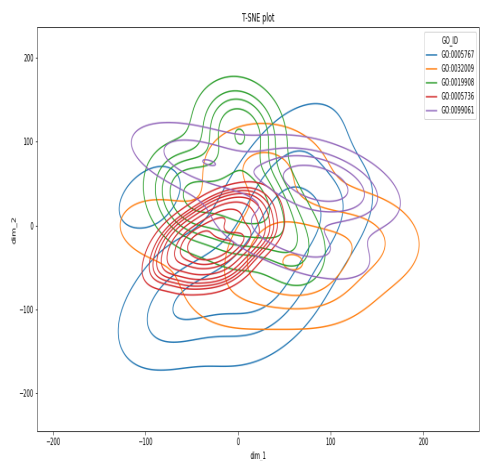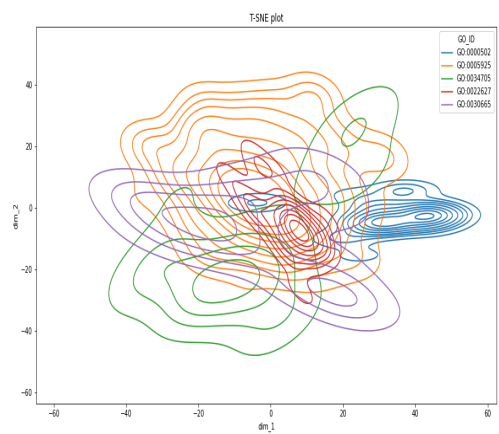

(g)

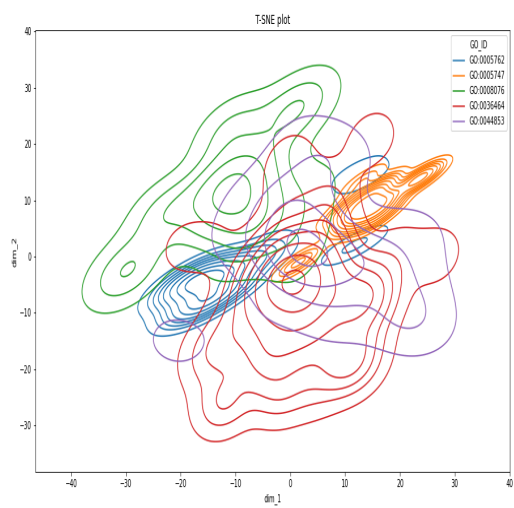

(h)

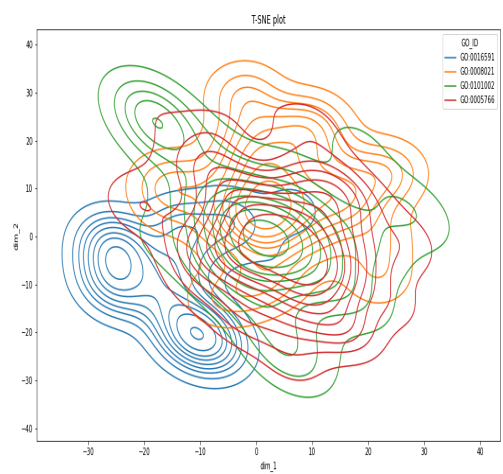

## Supplementary References

- Chen, Zhangguo, Lanfen Chen, Shuo-Wang Qiao, Takashi Nagaishi, and Richard S. Blumberg. 2008. "Carcinoembryonic Antigen-Related Cell Adhesion Molecule 1 Inhibits Proximal TCR Signaling by Targeting ZAP-70." *Journal of Immunology* 180 (9): 6085–93.
- Côté, A. L., P. Zhang, J. A. O'Sullivan, and V. L. Jacobs. 2011. "Stimulation of the Glucocorticoid-Induced TNF Receptor Family-Related Receptor on CD8 T Cells Induces Protective and High-Avidity T Cell Responses to Tumor ...." *The Journal of*.  
[https://journals.aai.org/jimmunol/article/186/1/275/39210?casa\\_token=kFyUVEIKzJQAAAAA:wtf4sNCIusBCVkl8hmURsOrUa5nYpJw5sGaUwTpaAdRkOCmNWRpyTKJ7ImAjkfsdzToNCsA](https://journals.aai.org/jimmunol/article/186/1/275/39210?casa_token=kFyUVEIKzJQAAAAA:wtf4sNCIusBCVkl8hmURsOrUa5nYpJw5sGaUwTpaAdRkOCmNWRpyTKJ7ImAjkfsdzToNCsA).
- Dam, Peter A. van, Yannick Verhoeven, Julie Jacobs, An Wouters, Wiebren Tjalma, Filip Lardon, Tim Van den Wyngaert, et al. 2019. "RANK-RANKL Signaling in Cancer of the Uterine Cervix: A Review." *International Journal of Molecular Sciences* 20 (9). <https://doi.org/10.3390/ijms20092183>.
- DeRosa, David C., Paul J. Ryan, Angela Okragly, Derrick R. Witcher, and Robert J. Benschop. 2008. "Tumor-Derived Death Receptor 6 Modulates Dendritic Cell Development." *Cancer Immunology, Immunotherapy: CII* 57 (6): 777–87.
- Dong, Mei, Tam How, Kellye C. Kirkbride, Kelly J. Gordon, Jason D. Lee, Nadine Hempel, Patrick Kelly, Benjamin J. Moeller, Jeffrey R. Marks, and Gerard C. Blobe. 1 2007. "The Type III TGF- $\beta$  Receptor Suppresses Breast Cancer Progression." *The Journal of Clinical Investigation* 117 (1): 206–17.
- Drenth, J. P., J. Göertz, M. R. Daha, and J. W. van der Meer. 1996. "Immunoglobulin D Enhances the Release of Tumor Necrosis Factor-Alpha, and Interleukin-1 Beta as Well as Interleukin-1 Receptor Antagonist from Human Mononuclear Cells." *Immunology* 88 (3): 355–62.
- Du, Peng, Ruihua Xiong, Xiaodong Li, and Jingting Jiang. 2016. "Immune Regulation and Antitumor Effect of TIM-1." *Journal of Immunology Research* 2016 (June):8605134.
- Durham, Nick M., Nick Holoweckyj, Randall S. MacGill, Kelly McGlinchey, Ching Ching Leow, and Scott H. Robbins. 2017. "GITR Ligand Fusion Protein Agonist Enhances the Tumor Antigen-specific CD8 T-Cell Response and Leads to Long-Lasting Memory." *Journal for ImmunoTherapy of Cancer* 5 (1): 47.
- Hao, Jing-Sheng, and Bao-En Shan. 2006. "Immune Enhancement and Anti-Tumour Activity of IL-23." *Cancer Immunology, Immunotherapy: CII* 55 (11): 1426–31.
- Hsieh, Shie-Liang, and Wan-Wan Lin. 2017. "Decoy Receptor 3: An Endogenous Immunomodulator in Cancer Growth and Inflammatory Reactions." *Journal of Biomedical Science* 24 (1): 39.
- Hu, Xiang, Yiding Bian, Xiaoli Wen, Mengfei Wang, Yiran Li, and Xiaoping Wan. 2020. "Collagen Triple Helix Repeat Containing 1 Promotes Endometrial Cancer Cell Migration by Activating the Focal Adhesion Kinase Signaling Pathway." *Experimental and Therapeutic Medicine* 20 (2): 1405–14.
- Ingermann, Angela R., Yong-Feng Yang, Jinfeng Han, Aki Mikami, Amanda E. Garza, Lathika Mohanraj, Lingbo Fan, et al. 2010. "Identification of a Novel Cell Death Receptor Mediating IGFBP-3-Induced Anti-Tumor Effects in Breast and Prostate Cancer." *The Journal of Biological Chemistry* 285 (39): 30233–46.
- Juric, Vladi, Chris O'Sullivan, Erin Stefanutti, Maria Kovalenko, Andrew Greenstein, Vivian Barry-Hamilton, Igor Mikaelian, et al. 2018. "MMP-9 Inhibition Promotes Anti-Tumor Immunity through Disruption of Biochemical and Physical Barriers to T-Cell Trafficking to Tumors." *PloS One* 13 (11): e0207255.
- Ju, Yunhe, Chuazheng Sun, and Xiaoli Wang. 2019. "Loss of Atypical Chemokine Receptor 4 Facilitates C-C Motif Chemokine Ligand 21-mediated Tumor Growth and Invasion in Nasopharyngeal Carcinoma." *Experimental and Therapeutic Medicine* 17 (1): 613–20.
- Lee, Jason D., Nadine Hempel, Nam Y. Lee, and Gerard C. Blobe. 2009. "The Type III TGF- $\beta$  Receptor Suppresses Breast Cancer Progression through GIPC-Mediated Inhibition of TGF- $\beta$  Signaling." *Carcinogenesis* 31 (2): 175–83.

- Leyland, R., A. Watkins, K. A. Mulgrew, and N. Holoweckyj. 2017. "A Novel Murine GITR Ligand Fusion Protein Induces Antitumor Activity as a Monotherapy That Is Further Enhanced in Combination with an OX40 Agonist Preclinical ...." *Clinical Cancer Research: An Official Journal of the American Association for Cancer Research*.  
<https://aacrjournals.org/clincancerres/article-abstract/23/13/3416/80061>.
- Li, Jing, Younghee Lee, Yanjian Li, Yu Jiang, Huiping Lu, Wenjuan Zang, Xiaohong Zhao, et al. 2018. "Co-Inhibitory Molecule B7 Superfamily Member 1 Expressed by Tumor-Infiltrating Myeloid Cells Induces Dysfunction of Anti-Tumor CD8<sup>+</sup> T Cells." *Immunity* 48 (4): 773–86.e5.
- Lin, Meng-Liang, and Shih-Shun Chen. 2017. "Activation of Casein Kinase II by Gallic Acid Induces BIK-BAX/BAK-Mediated ER Ca<sup>++</sup>-ROS-Dependent Apoptosis of Human Oral Cancer Cells." *Frontiers in Physiology* 8 (September):761.
- Li, Zhiyuan, Dan Li, Andy Tsun, and Bin Li. 2015. "FOXP3<sup>+</sup> Regulatory T Cells and Their Functional Regulation." *Cellular & Molecular Immunology* 12 (5): 558–65.
- Mebratu, Yohannes A., Ivan Leyva-Baca, Marc G. Wathelet, Neal Lacey, Hitendra S. Chand, Augustine M. K. Choi, and Yohannes Tesfaigzi. 2017. "Bik Reduces Hyperplastic Cells by Increasing Bak and Activating DAPk1 to Juxtapose ER and Mitochondria." *Nature Communications* 8 (1): 1–14.
- Mebratu, Yohannes A., Kurt Schwalm, Kevin R. Smith, Mark Schuyler, and Yohannes Tesfaigzi. 2011. "Cigarette Smoke Suppresses Bik To Cause Epithelial Cell Hyperplasia and Mucous Cell Metaplasia." *American Journal of Respiratory and Critical Care Medicine* 183 (11): 1531–38.
- Mei, Dan, Yue Zhu, Lingling Zhang, and Wei Wei. 2020. "The Role of CTHRC1 in Regulation of Multiple Signaling and Tumor Progression and Metastasis." *Mediators of Inflammation* 2020 (August):9578701.
- Parsi, Bahareh, Abolghasem Esmaeili, Mohammad Hashemi, and Mohaddeseh Behjati. 2016. "Transient Expression of Recombinant ACKR4 (CCRL1) Gene, an Atypical Chemokine Receptor in Human Embryonic Kidney (HEK 293) Cells." *Molecular Biology Reports* 43 (7): 583–89.
- Riese, David J., 2nd, and Richard L. Cullum. 2014. "Epregrulin: Roles in Normal Physiology and Cancer." *Seminars in Cell & Developmental Biology* 28 (April):49–56.
- Sumida, Kentaro, Yosuke Ohno, Junya Ohtake, Shun Kaneumi, Takuto Kishikawa, Norihiko Takahashi, Akinobu Taketomi, and Hidemitsu Kitamura. 2015. "IL-11 Induces Differentiation of Myeloid-Derived Suppressor Cells through Activation of STAT3 Signalling Pathway." *Scientific Reports* 5 (1): 1–10.
- Turley, Ryan S., Elizabeth C. Finger, Nadine Hempel, Tam How, Timothy A. Fields, and Gerard C. Blobe. 2007. "The Type III Transforming Growth Factor-Beta Receptor as a Novel Tumor Suppressor Gene in Prostate Cancer." *Cancer Research* 67 (3): 1090–98.
- Unsal, Serbulent, Heval Atas, Muammer Albayrak, Kemal Turhan, Aybar C. Acar, and Tunca Doğan. 2022. "Learning Functional Properties of Proteins with Language Models." *Nature Machine Intelligence* 4 (3): 227–45.
- Wang, Jia-Yu, and Wei-Peng Wang. 2020. "B7-H4, a Promising Target for Immunotherapy." *Cellular Immunology* 347 (January):104008.
- Whyte, Carly E., Maleika Osman, Ervin E. Kara, Caitlin Abbott, Jade Foeng, Duncan R. McKenzie, Kevin A. Fenix, et al. 2020. "ACKR4 Restrains Antitumor Immunity by Regulating CCL21." *The Journal of Experimental Medicine* 217 (6). <https://doi.org/10.1084/jem.20190634>.
- Yang, Xiao-Yan, Shigeyuki Ozawa, Yasumasa Kato, Yojiro Maehata, Kazuhito Izukuri, Takeharu Ikoma, Keisuke Kanamori, et al. 2019. "C-X-C Motif Chemokine Ligand 14 Is a Unique Multifunctional Regulator of Tumor Progression." *International Journal of Molecular Sciences* 20 (8).  
<https://doi.org/10.3390/ijms20081872>.
- Yu, Bo, Tianbo Jiang, and Delong Liu. 2020. "BCMA-Targeted Immunotherapy for Multiple Myeloma." *Journal of Hematology & Oncology* 13 (1): 125.
- Zhu, Han-Zhang, Wei-Jiang Zhou, Ya-Feng Wan, Ke Ge, Jun Lu, and Chang-Ku Jia. 2020.

“Downregulation of Orosomucoid 2 Acts as a Prognostic Factor Associated with Cancer-Promoting Pathways in Liver Cancer.” *World Journal of Gastroenterology: WJG* 26 (8): 804–17.
